# Supplementary material for: Fewer Steps, Better Plans: Sampling Variance in Flow-Matching Navigation World Models
Source: arXiv:2611.36153 source file (2026-11-26)
Supplement: Supplementary file 1 [file supp_axes_body.tex]

Depth + FFN & \M{1} & 0.44 & 65 & 0/12 & 12/12 & $+1.1$ & 0/12 & 12/12 & $+0.6$ \\
 & \M{4} & 1.00 & 132 & 1/12 & 12/12 & $+0.5$ & 0/12 & 12/12 & $+0.3$ \\
\addlinespace[2pt]
Heads + FFN & \M{1} & 0.27 & 46 & 1/12 & 12/12 & $+2.2$ & 1/12 & 12/12 & $+2.6$ \\
 & \M{4} & 1.00 & 109 & 0/12 & 12/12 & $+0.3$ & 1/12 & 12/12 & $+0.2$ \\
\addlinespace[2pt]
Heads + depth + FFN & \M{1} & 0.20 & 32 & 3/12 & 8/12 & $+4.0$ & 1/12 & 12/12 & $+3.8$ \\
 & \M{4} & 1.00 & 109 & 3/12 & 9/12 & $+0.8$ & 0/12 & 12/12 & $+0.6$ \\
\addlinespace[2pt]
Hidden width + FFN & \M{1} & 0.20 & 32 & 2/12 & 9/12 & $+5.5$ & 4/12 & 9/12 & $+5.5$ \\
 & \M{4} & 1.00 & 108 & 1/12 & 12/12 & $+0.7$ & 3/12 & 12/12 & $+0.1$ \\
\addlinespace[2pt]
Hidden width + depth + FFN & \M{1} & 0.14 & 21 & 3/12 & 8/12 & $+7.7$ & 5/12 & 9/12 & $+7.0$ \\
 & \M{4} & 1.00 & 110 & 3/12 & 10/12 & $+1.1$ & 1/12 & 12/12 & $+1.0$ \\
