# Supplementary material for: Fewer Steps, Better Plans: Sampling Variance in Flow-Matching Navigation World Models
Source: arXiv:2611.36153 source file (2026-11-26)
Supplement: Supplementary file 2 [file supp_axes_mid_body.tex]

Depth + FFN & \M{2} & 0.55 & 81 & 0/12 & 12/12 & $+0.6$ & 0/12 & 12/12 & $+0.6$ \\
 & \M{3} & 0.72 & 102 & 0/12 & 11/12 & $+0.4$ & 0/12 & 12/12 & $+0.5$ \\
\addlinespace[2pt]
Heads + FFN & \M{2} & 0.44 & 59 & 0/12 & 12/12 & $+0.7$ & 0/12 & 12/12 & $+0.8$ \\
 & \M{3} & 0.67 & 81 & 0/12 & 12/12 & $+0.3$ & 0/12 & 11/12 & $+0.5$ \\
\addlinespace[2pt]
Heads + depth + FFN & \M{2} & 0.36 & 47 & 2/12 & 8/12 & $+1.8$ & 0/12 & 12/12 & $+1.5$ \\
 & \M{3} & 0.61 & 73 & 2/12 & 9/12 & $+1.1$ & 0/12 & 11/12 & $+1.1$ \\
\addlinespace[2pt]
Hidden width + FFN & \M{2} & 0.35 & 47 & 0/12 & 10/12 & $+2.9$ & 2/12 & 12/12 & $+2.6$ \\
 & \M{3} & 0.59 & 72 & 0/12 & 10/12 & $+1.5$ & 1/12 & 12/12 & $+1.0$ \\
\addlinespace[2pt]
Hidden width + depth + FFN & \M{2} & 0.27 & 37 & 0/12 & 9/12 & $+4.0$ & 2/12 & 9/12 & $+4.0$ \\
 & \M{3} & 0.53 & 65 & 2/12 & 10/12 & $+2.0$ & 1/12 & 12/12 & $+2.2$ \\
