# Supplementary material for: Fewer Steps, Better Plans: Sampling Variance in Flow-Matching Navigation World Models
Source: arXiv:2611.36153 source file (2026-11-26)
Supplement: Supplementary file 3 [file supp_b0_curse_body.tex]

\sacson & \at{4}{50} & $100{\times}5$ & 0.0377 & 0.0426 & 0.88 & $+1.18$\sig \ci{$+1.06$, $+1.32$} & 49\,\% & 17\,\% & -- & 0.94 \ci{0.84, 1.04} \\
\sacson & \at{1}{50} & $500{\times}3$ & 0.0337 & 0.0374 & 0.90 & $+1.22$\sig \ci{$+1.16$, $+1.28$} & 49\,\% & 16\,\% & 1.00 (ref.) & 0.96 \ci{0.89, 1.03} \\
\sacson & \at{1}{5} & $500{\times}3{\times}3$ & 0.0268 & 0.0432 & 0.62 & $+0.73$\sig \ci{$+0.70$, $+0.77$} & 33\,\% & 27\,\% & 0.95 \ci{0.94, 0.95} & 0.94 \ci{0.87, 1.01} \\
\sacson & \at{1}{3} & $500{\times}2{\times}3$ & 0.0208 & 0.0469 & 0.44 & $+0.39$\sig \ci{$+0.37$, $+0.42$} & 20\,\% & 40\,\% & 0.86 \ci{0.85, 0.87} & 0.96 \ci{0.88, 1.05} \\
\sacson & \at{1}{2} & $500{\times}4{\times}3$ & 0.0118 & 0.0471 & 0.25 & $+0.08$\sig \ci{$+0.07$, $+0.09$} & 5\,\% & 68\,\% & 0.75 \ci{0.73, 0.76} & 0.90 \ci{0.83, 0.97} \\
\sacson & \M{1} Heun@3 & $100{\times}3$ & 0.0196 & 0.0416 & 0.47 & $+0.49$\sig \ci{$+0.42$, $+0.57$} & 24\,\% & 31\,\% & 0.96 \ci{0.96, 0.97} & -- \\
\sacson & \M{1} Midpoint@3 & $100{\times}3$ & 0.0245 & 0.0417 & 0.59 & $+0.76$\sig \ci{$+0.66$, $+0.87$} & 35\,\% & 22\,\% & 0.98 \ci{0.98, 0.99} & -- \\
\midrule
\recon & \at{1}{50} & $500{\times}3$ & 0.0257 & 0.0381 & 0.67 & $+1.21$\sig \ci{$+1.17$, $+1.26$} & 47\,\% & 13\,\% & 1.00 (ref.) & 1.39 \ci{1.30, 1.48} \\
\recon & \at{1}{5} & $500{\times}3{\times}3$ & 0.0206 & 0.0448 & 0.46 & $+0.69$\sig \ci{$+0.67$, $+0.71$} & 30\,\% & 22\,\% & 0.91 \ci{0.90, 0.91} & 1.39 \ci{1.30, 1.48} \\
\recon & \at{1}{3} & $500{\times}2{\times}3$ & 0.0145 & 0.0482 & 0.30 & $+0.36$\sig \ci{$+0.35$, $+0.38$} & 17\,\% & 33\,\% & 0.79 \ci{0.78, 0.81} & 1.43 \ci{1.33, 1.53} \\
\recon & \at{1}{2} & $500{\times}4{\times}3$ & 0.0046 & 0.0467 & 0.10 & $+0.04$\sig \ci{$+0.04$, $+0.04$} & 2\,\% & 68\,\% & 0.70 \ci{0.69, 0.72} & 1.39 \ci{1.30, 1.49} \\
\recon & \M{1} Heun@3 & $100{\times}3$ & 0.0179 & 0.0404 & 0.44 & $+0.67$\sig \ci{$+0.61$, $+0.73$} & 29\,\% & 24\,\% & 0.94 \ci{0.93, 0.95} & -- \\
\recon & \M{1} Midpoint@3 & $100{\times}3$ & 0.0219 & 0.0415 & 0.53 & $+0.81$\sig \ci{$+0.74$, $+0.88$} & 34\,\% & 20\,\% & 0.99 \ci{0.98, 0.99} & -- \\
\midrule
\scand & \at{1}{5} & $500{\times}3{\times}3$ & 0.0178 & 0.0479 & 0.37 & $+0.40$\sig \ci{$+0.38$, $+0.43$} & 20\,\% & 32\,\% & 1.00 (ref.) & 0.86 \ci{0.82, 0.91} \\
\scand & \at{1}{3} & $500{\times}2{\times}3$ & 0.0133 & 0.0487 & 0.27 & $+0.25$\sig \ci{$+0.23$, $+0.27$} & 14\,\% & 40\,\% & 0.93 \ci{0.93, 0.94} & 0.89 \ci{0.82, 0.96} \\
\scand & \at{1}{2} & $500{\times}4{\times}3$ & 0.0040 & 0.0463 & 0.09 & $+0.03$\sig \ci{$+0.03$, $+0.04$} & 2\,\% & 73\,\% & 0.83 \ci{0.82, 0.84} & 0.91 \ci{0.85, 0.97} \\
\scand & \M{1} Heun@3 & $100{\times}3$ & 0.0140 & 0.0467 & 0.30 & $+0.33$\sig \ci{$+0.28$, $+0.39$} & 18\,\% & 35\,\% & 0.86 \ci{0.85, 0.88} & -- \\
\scand & \M{1} Midpoint@3 & $100{\times}3$ & 0.0174 & 0.0502 & 0.35 & $+0.41$\sig \ci{$+0.36$, $+0.47$} & 21\,\% & 30\,\% & 0.89 \ci{0.87, 0.90} & -- \\
