# Supplementary material for: Fewer Steps, Better Plans: Sampling Variance in Flow-Matching Navigation World Models
Source: arXiv:2611.36153 source file (2026-11-26)
Supplement: Supplementary file 4 [file supp_b0_oneshot_body.tex]

\multicolumn{16}{@{}l}{\emph{1-shot direct prediction at 1\,s horizon (zero autoregressive chaining, full test splits: $3{,}416 / 4{,}262 / 1{,}883$ anchors)}} \\
\M{1}, $S{=}50$ (49) & 0.229 & 0.569 & 0.354 & 0.332 & 18.8 & 0.271 & 0.665 & 0.395 & 0.350 & 19.0 & 0.286 & 0.710 & 0.403 & 0.349 & 27.1 \\
\M{1}, $S{=}20$ (19) & 0.220 & 0.540 & 0.350 & 0.329 & 19.0 & 0.262 & 0.635 & 0.391 & 0.348 & 20.0 & 0.276 & 0.678 & 0.399 & 0.346 & 27.2 \\
\M{1}, $S{=}10$ (9) & 0.208 & 0.504 & 0.345 & 0.325 & 19.9 & 0.249 & 0.597 & 0.385 & 0.347 & 21.3 & 0.263 & 0.637 & 0.393 & 0.341 & 27.8 \\
\M{1}, $S{=}5$ (4) & 0.188 & 0.449 & 0.337 & 0.321 & 24.0 & 0.227 & 0.533 & 0.374 & 0.346 & 23.2 & 0.243 & 0.574 & 0.384 & 0.337 & 30.9 \\
\M{1}, $S{=}4$ (3) & 0.178 & 0.424 & 0.335 & 0.322 & 28.1 & 0.216 & 0.502 & 0.369 & 0.347 & 24.4 & 0.232 & 0.544 & 0.380 & 0.336 & 33.9 \\
\M{1}, $S{=}3$ (2) & 0.164 & 0.386 & 0.338 & 0.333 & 41.9 & 0.198 & 0.453 & 0.365 & 0.353 & 27.7 & 0.215 & 0.498 & 0.375 & 0.346 & 44.7 \\
\M{1}, $S{=}2$ (1) & 0.145 & 0.338 & 0.419 & 0.427 & 133.1 & 0.170 & 0.385 & 0.419 & 0.465 & 130.6 & 0.190 & 0.435 & 0.400 & 0.465 & 122.4 \\
\midrule
\multicolumn{16}{@{}l}{\emph{1-shot direct prediction at 4\,s horizon (zero autoregressive chaining; includes \mono $S{=}50{\to}2$ reference)}} \\
\mono, $S{=}50$ (49) & 0.223 & 0.553 & 0.345 & 0.323 & 16.5 & 0.287 & 0.703 & 0.413 & 0.374 & 18.9 & 0.335 & 0.834 & 0.458 & 0.405 & 28.5 \\
\mono, $S{=}5$ (4) & 0.184 & 0.442 & 0.326 & 0.310 & 20.5 & 0.244 & 0.576 & 0.392 & 0.369 & 21.7 & 0.296 & 0.702 & 0.444 & 0.397 & 33.3 \\
\mono, $S{=}3$ (2) & 0.160 & 0.379 & 0.323 & 0.319 & 32.7 & 0.213 & 0.489 & 0.383 & 0.376 & 25.1 & 0.268 & 0.615 & 0.439 & 0.406 & 49.9 \\
\mono, $S{=}2$ (1) & 0.140 & 0.327 & 0.400 & 0.408 & 112.2 & 0.181 & 0.408 & 0.448 & 0.485 & 140.3 & 0.239 & 0.536 & 0.473 & 0.526 & 146.4 \\
\midrule
\M{1}, $S{=}50$ (49) & 0.235 & 0.582 & 0.362 & 0.343 & 19.1 & 0.295 & 0.722 & 0.422 & 0.385 & 20.3 & 0.334 & 0.828 & 0.456 & 0.399 & 31.1 \\
\M{1}, $S{=}5$ (4) & 0.192 & 0.458 & 0.344 & 0.331 & 24.7 & 0.249 & 0.583 & 0.401 & 0.382 & 25.0 & 0.289 & 0.679 & 0.440 & 0.389 & 36.4 \\
\M{1}, $S{=}3$ (2) & 0.168 & 0.393 & 0.346 & 0.344 & 44.7 & 0.218 & 0.496 & 0.393 & 0.389 & 31.0 & 0.259 & 0.590 & 0.433 & 0.401 & 55.1 \\
\M{1}, $S{=}2$ (1) & 0.148 & 0.346 & 0.438 & 0.442 & 141.8 & 0.186 & 0.419 & 0.469 & 0.510 & 172.3 & 0.229 & 0.515 & 0.476 & 0.547 & 169.7 \\
