# Supplementary material for: Fewer Steps, Better Plans: Sampling Variance in Flow-Matching Navigation World Models
Source: arXiv:2611.36153 source file (2026-11-26)
Supplement: Supplementary file 5 [file supp_b2_cal_body.tex]

\monoat{50} & 49 & $2.154\pm0.023$ & $0.612\pm0.010$\sig & $-0.087$\sig \ci{$-0.173$, $-0.001$} & 1.56 & 1.80 & 2.06 & 3.19 & 1.42 / 1.41 \\
\at{4}{50} & 49 & $2.209\pm0.059$ & $0.617\pm0.011$\sig & $-0.032$ \ci{$-0.120$, $+0.055$} & 1.62 & 1.86 & 2.13 & 3.22 & 1.47 / 1.44 \\
\at{1}{50} & 49 & $2.229\pm0.037$ & $0.619\pm0.007$\sig & $-0.012$ \ci{$-0.101$, $+0.077$} & 1.71 & 1.86 & 2.13 & 3.22 & 1.53 / 1.41 \\
Standalone \M{0}@50 & 49 & $2.348\pm0.042$ & $0.634\pm0.009$\sig & $+0.107$\sig \ci{$+0.023$, $+0.193$} & 1.77 & 1.95 & 2.28 & 3.39 & 1.59 / 1.49 \\
\midrule
\monoat{5} & 4 & $2.091\pm0.041$ & $0.601\pm0.002$ & $-0.150$\sig$^{\ddagger}$ \ci{$-0.240$, $-0.061$} & 1.54 & 1.76 & 1.96 & 3.11 & 1.38 / 1.37 \\
\at{4}{5} & 4 & $2.100\pm0.045$ & $0.600\pm0.006$ & $-0.141$\sig$^{\ddagger}$ \ci{$-0.228$, $-0.054$} & 1.50 & 1.73 & 2.02 & 3.15 & 1.40 / 1.36 \\
\at{1}{5} & 4 & $2.130\pm0.041$ & $0.606\pm0.004$\sig & $-0.111$\sig \ci{$-0.205$, $-0.020$} & 1.52 & 1.80 & 2.07 & 3.13 & 1.45 / 1.36 \\
Standalone \M{0}@5 & 4 & $2.244\pm0.052$ & $0.622\pm0.008$\sig & $+0.004$ \ci{$-0.089$, $+0.094$} & 1.68 & 1.86 & 2.15 & 3.29 & 1.52 / 1.43 \\
\midrule
\mono Heun@3 & 4 & $2.131\pm0.020$ & $0.600\pm0.012$ & $-0.110$\sig \ci{$-0.202$, $-0.020$} & 1.61 & 1.80 & 2.04 & 3.08 & 1.44 / 1.37 \\
\mono Midpoint@3 & 4 & $2.161\pm0.031$ & $0.606\pm0.009$\sig & $-0.080$ \ci{$-0.169$, $+0.011$} & 1.63 & 1.84 & 2.04 & 3.13 & 1.43 / 1.41 \\
\M{1} Heun@3 & 4 & $2.204\pm0.043$ & $0.611\pm0.012$\sig & $-0.037$ \ci{$-0.131$, $+0.058$} & 1.66 & 1.87 & 2.13 & 3.16 & 1.54 / 1.35 \\
\M{1} Midpoint@3 & 4 & $2.153\pm0.064$ & $0.603\pm0.009$ & $-0.088$ \ci{$-0.182$, $+0.008$} & 1.57 & 1.78 & 2.10 & 3.16 & 1.48 / 1.35 \\
\midrule
\monoat{3} & 2 & $2.084\pm0.017$ & $0.601\pm0.008$ & $-0.157$\sig$^{\ddagger}$ \ci{$-0.251$, $-0.065$} & 1.48 & 1.79 & 2.01 & 3.06 & 1.40 / 1.34 \\
\at{4}{3} & 2 & $2.106\pm0.011$ & $0.604\pm0.005$\sig & $-0.135$\sig$^{\ddagger}$ \ci{$-0.226$, $-0.045$} & 1.48 & 1.76 & 2.11 & 3.08 & 1.44 / 1.32 \\
\at{1}{3} & 2 & $2.142\pm0.044$ & $0.613\pm0.006$\sig & $-0.099$\sig \ci{$-0.192$, $-0.007$} & 1.52 & 1.79 & 2.14 & 3.13 & 1.50 / 1.31 \\
\midrule
$2{\times}\monoat{3}$ & 2$\times$2 & $2.057\pm0.038$ & $0.600\pm0.008$ & $-0.184$\sig$^{\ddagger}$ \ci{$-0.281$, $-0.087$} & 1.46 & 1.79 & 1.95 & 3.02 & 1.39 / 1.32 \\
$2{\times}\at{4}{3}$ & 2$\times$2 & $2.079\pm0.028$ & $0.600\pm0.008$ & $-0.162$\sig$^{\ddagger}$ \ci{$-0.253$, $-0.071$} & 1.47 & 1.75 & 2.06 & 3.04 & 1.44 / 1.29 \\
$2{\times}\at{1}{3}$ & 2$\times$2 & $2.092\pm0.029$ & $0.602\pm0.003$ & $-0.149$\sig$^{\ddagger}$ \ci{$-0.244$, $-0.055$} & 1.48 & 1.78 & 2.04 & 3.07 & 1.45 / 1.30 \\
\midrule
\monoat{2} & 1 & $2.182\pm0.018$ & $0.620\pm0.004$\sig & $-0.059$ \ci{$-0.162$, $+0.041$} & 1.65 & 1.99 & 1.99 & 3.09 & 1.53 / 1.32 \\
\at{4}{2} & 1 & $2.138\pm0.038$ & $0.610\pm0.008$\sig & $-0.103$\sig \ci{$-0.198$, $-0.007$} & 1.58 & 1.81 & 2.08 & 3.09 & 1.54 / 1.25 \\
\at{1}{2} & 1 & $2.249\pm0.023$ & $0.631\pm0.003$\sig & $+0.008$ \ci{$-0.093$, $+0.107$} & 1.70 & 1.92 & 2.15 & 3.23 & 1.65 / 1.28 \\
\midrule
$4{\times}\monoat{2}$ & 4$\times$1 & $2.198\pm0.010$ & $0.621\pm0.006$\sig & $-0.043$ \ci{$-0.144$, $+0.056$} & 1.67 & 1.97 & 2.04 & 3.11 & 1.56 / 1.32 \\
$4{\times}\at{4}{2}$ & 4$\times$1 & $2.142\pm0.037$ & $0.609\pm0.004$\sig & $-0.099$\sig \ci{$-0.194$, $-0.005$} & 1.58 & 1.82 & 2.07 & 3.11 & 1.54 / 1.26 \\
$4{\times}\at{1}{2}$ & 4$\times$1 & $2.253\pm0.039$ & $0.632\pm0.004$\sig & $+0.013$ \ci{$-0.087$, $+0.111$} & 1.68 & 1.95 & 2.18 & 3.20 & 1.65 / 1.28 \\
\midrule
Straight line (train-fit $v_0{=}0.896$) & -- & 2.241 & 0.585 & -- & 1.19 & 1.65 & 2.31 & 3.82 & 1.60 / 1.28 \\
\cem prior mean (calibrated) & -- & 2.241 & 0.585 & -- & 1.19 & 1.65 & 2.31 & 3.82 & 1.60 / 1.28 \\
Random shooting (calibrated) & -- & 2.800 & 0.737 & -- & 2.08 & 2.31 & 2.75 & 4.06 & 1.92 / 1.72 \\
Oracle (mean of 3 best of 120) & -- & 0.690 & 0.384 & -- & 0.47 & 0.53 & 0.63 & 1.13 & 0.46 / 0.48 \\
