# Supplementary material for: Fewer Steps, Better Plans: Sampling Variance in Flow-Matching Navigation World Models
Source: arXiv:2611.36153 source file (2026-11-26)
Supplement: Supplementary file 6 [file supp_calibration_body.tex]

Zero motion & 5.081 & 5.161 & 4.930 \\
\cem prior mean (straight line) & 1.637 & 3.780 & 0.834 \\
Straight line at train-split mean progress (one scalar) & 1.589 & 2.241 & 0.834 \\
\midrule
Random shooting (mean of 3 random candidates; 20 repetitions) & 1.77 & 4.07 & 1.08 \\
Oracle: best fresh candidate & 0.617 $\pm$ 0.005 & 1.186 $\pm$ 0.014 & 0.334 $\pm$ 0.004 \\
Oracle: mean of the 3 best fresh candidates & 0.61 & 1.08 & 0.27 \\
\midrule
\monoat{50} & 1.351 & 2.847 & 1.012 \\
\at{1}{50} & 1.371 & 2.777 & 1.014 \\
\monoat{5} & 1.294 & 2.777 & 1.007 \\
\at{4}{5} & 1.270 & 2.712 & 0.997 \\
\at{1}{5} & 1.259 & 2.676 & 1.000 \\
