# Supplementary material for: Fewer Steps, Better Plans: Sampling Variance in Flow-Matching Navigation World Models
Source: arXiv:2611.36153 source file (2026-11-26)
Supplement: Supplementary file 7 [file supp_cluster_body.tex]

\M{1} $-$ \mono & 50 & \recon & $+0.020$ & [$-0.021$, $+0.065$] & [$-0.023$, $+0.060$] & 391 \\
\M{1} $-$ \mono & 50 & \sacson & $-0.070$ & [$-0.163$, $+0.015$] & [$-0.169$, $+0.025$] & 202 \\
\M{1} $-$ \mono & 50 & \scand & $+0.002$ & [$-0.038$, $+0.042$] & [$-0.042$, $+0.047$] & 43 \\
\midrule
\M{4} $-$ \mono & 50 & \recon & $+0.025$ & [$-0.016$, $+0.067$] & [$-0.019$, $+0.068$] & 391 \\
\M{4} $-$ \mono & 50 & \sacson & $-0.042$ & [$-0.131$, $+0.048$] & [$-0.125$, $+0.046$] & 202 \\
\M{4} $-$ \mono & 50 & \scand & $+0.012$ & [$-0.025$, $+0.052$] & [$-0.031$, $+0.054$] & 43 \\
\midrule
\M{1} $-$ \M{4} & 50 & \recon & $-0.005$ & [$-0.043$, $+0.032$] & [$-0.040$, $+0.031$] & 391 \\
\M{1} $-$ \M{4} & 50 & \sacson & $-0.028$ & [$-0.103$, $+0.044$] & [$-0.105$, $+0.049$] & 202 \\
\M{1} $-$ \M{4} & 50 & \scand & $-0.010$ & [$-0.047$, $+0.026$] & [$-0.049$, $+0.026$] & 43 \\
\midrule
\M{1} $-$ \mono & 5 & \recon & $-0.035$ & [$-0.076$, $+0.003$] & [$-0.074$, $+0.004$] & 391 \\
\M{1} $-$ \mono & 5 & \sacson & $-0.101$ & [$-0.187$, $-0.015$] & [$-0.190$, $-0.013$] & 202 \\
\M{1} $-$ \mono & 5 & \scand & $-0.007$ & [$-0.051$, $+0.036$] & [$-0.054$, $+0.035$] & 43 \\
\midrule
\M{4} $-$ \mono & 5 & \recon & $-0.024$ & [$-0.063$, $+0.013$] & [$-0.062$, $+0.016$] & 391 \\
\M{4} $-$ \mono & 5 & \sacson & $-0.065$ & [$-0.156$, $+0.021$] & [$-0.150$, $+0.022$] & 202 \\
\M{4} $-$ \mono & 5 & \scand & $-0.010$ & [$-0.052$, $+0.032$] & [$-0.057$, $+0.031$] & 43 \\
\midrule
\M{1} $-$ \M{4} & 5 & \recon & $-0.011$ & [$-0.041$, $+0.021$] & [$-0.041$, $+0.021$] & 391 \\
\M{1} $-$ \M{4} & 5 & \sacson & $-0.036$ & [$-0.105$, $+0.035$] & [$-0.106$, $+0.033$] & 202 \\
\M{1} $-$ \M{4} & 5 & \scand & $+0.003$ & [$-0.033$, $+0.038$] & [$-0.038$, $+0.045$] & 43 \\
\midrule
\M{1} $-$ \mono & 3 & \recon & $-0.028$ & [$-0.065$, $+0.008$] & [$-0.066$, $+0.010$] & 391 \\
\M{1} $-$ \mono & 3 & \sacson & $-0.056$ & [$-0.150$, $+0.034$] & [$-0.150$, $+0.036$] & 202 \\
\M{1} $-$ \mono & 3 & \scand & $-0.061$ & [$-0.104$, $-0.016$] & [$-0.105$, $-0.019$] & 43 \\
\midrule
\M{4} $-$ \mono & 3 & \recon & $-0.021$ & [$-0.054$, $+0.011$] & [$-0.055$, $+0.013$] & 391 \\
\M{4} $-$ \mono & 3 & \sacson & $-0.037$ & [$-0.129$, $+0.056$] & [$-0.148$, $+0.064$] & 202 \\
\M{4} $-$ \mono & 3 & \scand & $-0.068$ & [$-0.113$, $-0.022$] & [$-0.109$, $-0.025$] & 43 \\
\midrule
\M{1} $-$ \M{4} & 3 & \recon & $-0.007$ & [$-0.038$, $+0.023$] & [$-0.039$, $+0.024$] & 391 \\
\M{1} $-$ \M{4} & 3 & \sacson & $-0.019$ & [$-0.091$, $+0.049$] & [$-0.093$, $+0.056$] & 202 \\
\M{1} $-$ \M{4} & 3 & \scand & $+0.007$ & [$-0.025$, $+0.038$] & [$-0.017$, $+0.037$] & 43 \\
\midrule
\at{1}{5} $-$ \at{1}{50} & 5/50 & \recon & $-0.112$ & [$-0.154$, $-0.072$] & [$-0.155$, $-0.073$] & 391 \\
\at{1}{5} $-$ \at{1}{50} & 5/50 & \sacson & $-0.101$ & [$-0.172$, $-0.023$] & [$-0.181$, $-0.017$] & 202 \\
\at{1}{5} $-$ \at{1}{50} & 5/50 & \scand & $-0.014$ & [$-0.053$, $+0.025$] & [$-0.054$, $+0.031$] & 43 \\
\midrule
\monoat{5} $-$ \monoat{50} & 5/50 & \recon & $-0.057$ & [$-0.097$, $-0.016$] & [$-0.095$, $-0.022$] & 391 \\
\monoat{5} $-$ \monoat{50} & 5/50 & \sacson & $-0.070$ & [$-0.149$, $+0.008$] & [$-0.148$, $+0.011$] & 202 \\
\monoat{5} $-$ \monoat{50} & 5/50 & \scand & $-0.004$ & [$-0.040$, $+0.029$] & [$-0.041$, $+0.033$] & 43 \\
