# Supplementary material for: Fewer Steps, Better Plans: Sampling Variance in Flow-Matching Navigation World Models
Source: arXiv:2611.36153 source file (2026-11-26)
Supplement: Supplementary file 8 [file supp_difficulty_body.tex]

\recon & near prior & 1.025 & 1.045 & 0.991 & 0.982 & $-0.035$\sig [$-0.066$, $-0.005$] & $-0.053$\sig [$-0.084$, $-0.021$] & $-0.063$\sig [$-0.102$, $-0.023$] \\
 & far from prior & 2.249 & 1.681 & 1.600 & 1.551 & $-0.168$\sig [$-0.206$, $-0.129$] & $-0.081$\sig [$-0.115$, $-0.050$] & $-0.130$\sig [$-0.173$, $-0.087$] \\
\midrule
\sacson & near prior & 2.325 & 1.669 & 1.603 & 1.600 & $-0.076$\sig [$-0.133$, $-0.013$] & $-0.066$\sig [$-0.120$, $-0.015$] & $-0.069$\sig [$-0.140$, $-0.004$] \\
 & far from prior & 5.234 & 4.006 & 3.910 & 3.897 & $-0.099$\sig [$-0.179$, $-0.022$] & $-0.096$\sig [$-0.176$, $-0.019$] & $-0.109$\sig [$-0.213$, $-0.010$] \\
\midrule
\scand & near prior & 0.371 & 0.670 & 0.676 & 0.661 & $-0.012$ [$-0.039$, $+0.016$] & $+0.006$ [$-0.019$, $+0.032$] & $-0.009$ [$-0.037$, $+0.020$] \\
 & far from prior & 1.297 & 1.405 & 1.387 & 1.360 & $-0.018$ [$-0.053$, $+0.017$] & $-0.018$ [$-0.054$, $+0.016$] & $-0.045$\sig [$-0.086$, $-0.004$] \\
