# Supplementary material for: Fewer Steps, Better Plans: Sampling Variance in Flow-Matching Navigation World Models
Source: arXiv:2611.36153 source file (2026-11-26)
Supplement: Supplementary file 9 [file supp_e12_body.tex]

\multicolumn{7}{@{}l}{\emph{\paper \M{1} ($500$ items per dataset)}} \\
$S{=}20 - S{=}50$ (19 vs.\ 49 NFEs) & $-0.027$ [$-0.053$, $+0.001$] & $-0.021$\sig [$-0.037$, $-0.005$] & $+0.013$ [$-0.028$, $+0.059$] & $-0.002$ [$-0.027$, $+0.028$] & $+0.002$ [$-0.026$, $+0.028$] & $+0.010$ [$-0.004$, $+0.026$] \\
$S{=}10 - S{=}50$ (9 vs.\ 49 NFEs) & $-0.052$\sig [$-0.082$, $-0.020$] & $-0.056$\sig [$-0.076$, $-0.036$] & $-0.036$ [$-0.091$, $+0.025$] & $-0.060$\sig [$-0.094$, $-0.022$] & $-0.022$ [$-0.056$, $+0.010$] & $-0.010$ [$-0.030$, $+0.008$] \\
$S{=}4 - S{=}5$ (3 vs.\ 4 NFEs) & $+0.009$ [$-0.014$, $+0.033$] & $-0.004$ [$-0.019$, $+0.009$] & $-0.010$ [$-0.067$, $+0.044$] & $-0.035$ [$-0.066$, $+0.000$] & $+0.001$ [$-0.029$, $+0.030$] & $-0.003$ [$-0.018$, $+0.012$] \\
$S{=}4 - S{=}3$ (3 vs.\ 2 NFEs) & $+0.025$ [$-0.001$, $+0.052$] & $+0.015$ [$-0.000$, $+0.031$] & $-0.007$ [$-0.064$, $+0.048$] & $-0.001$ [$-0.040$, $+0.035$] & $-0.012$ [$-0.045$, $+0.018$] & $+0.010$ [$-0.007$, $+0.029$] \\
$S{=}10 - S{=}5$ (9 vs.\ 4 NFEs) & $+0.060$\sig [$+0.028$, $+0.092$] & $+0.045$\sig [$+0.029$, $+0.064$] & $+0.065$\sig [$+0.000$, $+0.130$] & $+0.027$ [$-0.012$, $+0.065$] & $-0.009$ [$-0.044$, $+0.028$] & $+0.006$ [$-0.014$, $+0.025$] \\
Unif.\ Euler ($\alpha{=}1$) $-$ shifted Euler ($S{=}5$, 4 NFEs) & $+0.016$ [$-0.022$, $+0.056$] & $+0.016$ [$-0.007$, $+0.040$] & $+0.025$ [$-0.056$, $+0.117$] & $-0.015$ [$-0.069$, $+0.049$] & $-0.009$ [$-0.047$, $+0.031$] & $-0.008$ [$-0.029$, $+0.014$] \\
Unif.\ Euler ($\alpha{=}1$) $-$ unif.\ Heun ($\alpha{=}1$, 4 NFEs) & $-0.058$\sig [$-0.094$, $-0.025$] & $-0.054$\sig [$-0.075$, $-0.033$] & $-0.045$ [$-0.111$, $+0.026$] & $-0.019$ [$-0.057$, $+0.020$] & $-0.019$ [$-0.052$, $+0.016$] & $-0.022$\sig [$-0.041$, $-0.001$] \\
Unif.\ Euler ($\alpha{=}1$) $-$ unif.\ midpoint ($\alpha{=}1$, 4 NFEs) & $-0.085$\sig [$-0.122$, $-0.045$] & $-0.092$\sig [$-0.115$, $-0.069$] & $-0.048$ [$-0.120$, $+0.027$] & $-0.011$ [$-0.051$, $+0.032$] & $-0.020$ [$-0.060$, $+0.019$] & $-0.025$\sig [$-0.047$, $-0.004$] \\
\midrule
\multicolumn{7}{@{}l}{\emph{\mono ($500$ items per dataset)}} \\
$S{=}20 - S{=}50$ (19 vs.\ 49 NFEs) & $-0.002$ [$-0.027$, $+0.026$] & $-0.012$ [$-0.028$, $+0.003$] & $+0.002$ [$-0.046$, $+0.049$] & $-0.021$ [$-0.050$, $+0.007$] & $+0.015$ [$-0.008$, $+0.038$] & $+0.009$ [$-0.005$, $+0.021$] \\
$S{=}10 - S{=}50$ (9 vs.\ 49 NFEs) & $-0.026$ [$-0.058$, $+0.007$] & $-0.033$\sig [$-0.052$, $-0.013$] & $-0.047$ [$-0.114$, $+0.005$] & $-0.064$\sig [$-0.098$, $-0.029$] & $-0.016$ [$-0.045$, $+0.010$] & $-0.009$ [$-0.027$, $+0.009$] \\
$S{=}4 - S{=}5$ (3 vs.\ 4 NFEs) & $-0.007$ [$-0.037$, $+0.020$] & $-0.011$ [$-0.026$, $+0.004$] & $-0.059$\sig [$-0.111$, $-0.006$] & $-0.059$\sig [$-0.090$, $-0.026$] & $+0.031$\sig [$+0.007$, $+0.055$] & $+0.001$ [$-0.013$, $+0.016$] \\
$S{=}4 - S{=}3$ (3 vs.\ 2 NFEs) & $+0.016$ [$-0.012$, $+0.043$] & $+0.013$ [$-0.004$, $+0.031$] & $-0.011$ [$-0.071$, $+0.048$] & $+0.036$ [$-0.001$, $+0.072$] & $-0.037$\sig [$-0.068$, $-0.003$] & $-0.025$\sig [$-0.043$, $-0.007$] \\
$S{=}10 - S{=}5$ (9 vs.\ 4 NFEs) & $+0.031$\sig [$+0.003$, $+0.060$] & $+0.035$\sig [$+0.016$, $+0.053$] & $+0.023$ [$-0.051$, $+0.092$] & $+0.017$ [$-0.028$, $+0.057$] & $-0.012$ [$-0.041$, $+0.018$] & $-0.003$ [$-0.020$, $+0.016$] \\
Unif.\ Euler ($\alpha{=}1$) $-$ shifted Euler ($S{=}5$, 4 NFEs) & $+0.008$ [$-0.027$, $+0.043$] & $+0.013$ [$-0.015$, $+0.039$] & $-0.029$ [$-0.109$, $+0.056$] & $-0.071$\sig [$-0.118$, $-0.019$] & $+0.001$ [$-0.035$, $+0.036$] & $+0.006$ [$-0.015$, $+0.028$] \\
Unif.\ Euler ($\alpha{=}1$) $-$ unif.\ Heun ($\alpha{=}1$, 4 NFEs) & $-0.041$\sig [$-0.074$, $-0.010$] & $-0.045$\sig [$-0.067$, $-0.023$] & $+0.015$ [$-0.052$, $+0.079$] & $-0.028$ [$-0.068$, $+0.006$] & $+0.001$ [$-0.029$, $+0.030$] & $-0.002$ [$-0.020$, $+0.017$] \\
Unif.\ Euler ($\alpha{=}1$) $-$ unif.\ midpoint ($\alpha{=}1$, 4 NFEs) & $-0.064$\sig [$-0.099$, $-0.029$] & $-0.078$\sig [$-0.103$, $-0.056$] & $-0.046$ [$-0.112$, $+0.021$] & $-0.042$ [$-0.084$, $+0.001$] & $-0.032$\sig [$-0.062$, $-0.002$] & $-0.010$ [$-0.030$, $+0.010$] \\
