# Supplementary material for: Fewer Steps, Better Plans: Sampling Variance in Flow-Matching Navigation World Models
Source: arXiv:2611.36153 source file (2026-11-26)
Supplement: Supplementary file 10 [file supp_gen_full_body.tex]

\M{1} & 50 & 0.385 & 0.422 & 20.3 & 0.343 & 0.362 & 19.1 & 0.399 & 0.456 & 31.1 \\
 & 20 & 0.383 & 0.418 & 21.3 & 0.340 & 0.358 & 19.1 & 0.396 & 0.453 & 31.5 \\
 & 10 & 0.382 & 0.412 & 22.7 & 0.335 & 0.352 & 20.1 & 0.393 & 0.448 & 32.5 \\
 & 7 & 0.382 & 0.407 & 23.7 & 0.333 & 0.348 & 21.4 & 0.391 & 0.444 & 33.7 \\
 & 5 & 0.382 & 0.401 & 25.0 & 0.331 & 0.344 & 24.7 & 0.389 & 0.440 & 36.4 \\
 & 4 & 0.383 & 0.396 & 26.4 & 0.333 & 0.342 & 29.5 & 0.390 & 0.436 & 40.5 \\
 & 3 & 0.389 & 0.393 & 31.0 & 0.344 & 0.346 & 44.7 & 0.401 & 0.433 & 55.1 \\
 & 2 & 0.510 & 0.469 & 172.5 & 0.442 & 0.438 & 142.0 & 0.547 & 0.476 & 169.7 \\
\midrule
\M{2} & 50 & 0.382 & 0.420 & 19.6 & 0.340 & 0.358 & 18.2 & 0.399 & 0.456 & 30.5 \\
 & 20 & 0.380 & 0.416 & 20.5 & 0.336 & 0.354 & 18.3 & 0.396 & 0.453 & 30.8 \\
 & 10 & 0.379 & 0.410 & 21.7 & 0.332 & 0.348 & 19.3 & 0.393 & 0.447 & 31.6 \\
 & 5 & 0.379 & 0.399 & 23.6 & 0.327 & 0.340 & 23.6 & 0.389 & 0.439 & 35.4 \\
 & 3 & 0.387 & 0.390 & 29.0 & 0.338 & 0.341 & 41.9 & 0.400 & 0.432 & 53.8 \\
\midrule
\M{3} & 50 & 0.381 & 0.419 & 19.4 & 0.336 & 0.356 & 17.6 & 0.399 & 0.455 & 29.6 \\
 & 20 & 0.379 & 0.415 & 20.2 & 0.332 & 0.352 & 17.7 & 0.396 & 0.452 & 29.9 \\
 & 10 & 0.378 & 0.409 & 21.3 & 0.328 & 0.346 & 18.6 & 0.393 & 0.447 & 30.6 \\
 & 5 & 0.377 & 0.397 & 23.3 & 0.324 & 0.337 & 22.5 & 0.389 & 0.438 & 34.4 \\
 & 3 & 0.384 & 0.388 & 27.9 & 0.333 & 0.337 & 39.3 & 0.398 & 0.431 & 52.8 \\
\midrule
\M{4} & 50 & 0.379 & 0.418 & 19.1 & 0.333 & 0.354 & 17.1 & 0.399 & 0.455 & 29.1 \\
 & 20 & 0.378 & 0.414 & 20.0 & 0.330 & 0.349 & 17.3 & 0.397 & 0.451 & 29.4 \\
 & 10 & 0.376 & 0.408 & 20.8 & 0.326 & 0.344 & 18.2 & 0.393 & 0.446 & 30.3 \\
 & 7 & 0.376 & 0.403 & 21.8 & 0.323 & 0.340 & 19.2 & 0.391 & 0.442 & 31.5 \\
 & 5 & 0.375 & 0.397 & 22.9 & 0.320 & 0.335 & 21.6 & 0.389 & 0.438 & 34.1 \\
 & 4 & 0.376 & 0.392 & 24.2 & 0.320 & 0.332 & 25.3 & 0.388 & 0.434 & 37.8 \\
 & 3 & 0.382 & 0.387 & 27.6 & 0.329 & 0.334 & 37.1 & 0.398 & 0.431 & 52.1 \\
 & 2 & 0.495 & 0.457 & 154.1 & 0.422 & 0.416 & 124.8 & 0.537 & 0.471 & 163.6 \\
\midrule
\mono & 50 & 0.374 & 0.413 & 18.9 & 0.323 & 0.345 & 16.5 & 0.405 & 0.458 & 28.5 \\
 & 20 & 0.372 & 0.409 & 19.3 & 0.320 & 0.341 & 16.7 & 0.403 & 0.455 & 28.9 \\
 & 10 & 0.370 & 0.403 & 20.1 & 0.316 & 0.335 & 17.4 & 0.401 & 0.451 & 29.8 \\
 & 7 & 0.370 & 0.398 & 20.7 & 0.313 & 0.331 & 18.5 & 0.399 & 0.448 & 30.9 \\
 & 5 & 0.369 & 0.392 & 21.7 & 0.310 & 0.326 & 20.5 & 0.397 & 0.444 & 33.3 \\
 & 4 & 0.370 & 0.387 & 22.7 & 0.310 & 0.323 & 23.3 & 0.397 & 0.441 & 36.8 \\
 & 3 & 0.376 & 0.383 & 25.1 & 0.319 & 0.323 & 32.7 & 0.406 & 0.439 & 49.9 \\
 & 2 & 0.485 & 0.448 & 140.5 & 0.408 & 0.400 & 112.4 & 0.526 & 0.473 & 146.4 \\
\midrule
\mono, naive \M{1} slice & 50 & 0.939 & 0.866 & 494.2 & 0.873 & 0.847 & 408.0 & 0.933 & 0.889 & 444.3 \\
 & 5 & 0.795 & 0.877 & 432.5 & 0.825 & 0.859 & 442.3 & 0.900 & 0.887 & 439.1 \\
\midrule
Standalone \M{1} & 50 & 0.381 & 0.418 & 20.3 & 0.334 & 0.354 & 17.7 & 0.401 & 0.457 & 30.1 \\
 & 5 & 0.378 & 0.397 & 23.9 & 0.322 & 0.336 & 22.7 & 0.392 & 0.440 & 35.8 \\
\midrule
Standalone \M{0} & 50 & 0.399 & 0.432 & 21.3 & 0.358 & 0.374 & 20.9 & 0.408 & 0.465 & 33.6 \\
 & 5 & 0.397 & 0.411 & 26.2 & 0.345 & 0.358 & 27.4 & 0.398 & 0.448 & 41.1 \\
