# Supplementary material for: Fewer Steps, Better Plans: Sampling Variance in Flow-Matching Navigation World Models
Source: arXiv:2611.36153 source file (2026-11-26)
Supplement: Supplementary file 11 [file supp_gen_horizon_body.tex]

\recon & \M{1} & 50 & 0.350 & 0.366 & 0.385 & 0.407 & 0.460 & 19.0 & 19.5 & 20.3 & 21.3 & 20.3 \\
\recon & \M{1} & 5 & 0.346 & 0.362 & 0.382 & 0.406 & 0.463 & 23.2 & 24.0 & 25.0 & 26.5 & 25.0 \\
\recon & \M{2} & 50 & 0.348 & 0.363 & 0.382 & 0.404 & 0.458 & 18.5 & 18.8 & 19.6 & 20.5 & 19.7 \\
\recon & \M{2} & 5 & 0.343 & 0.360 & 0.379 & 0.403 & 0.460 & 22.4 & 22.8 & 23.6 & 25.0 & 23.9 \\
\recon & \M{3} & 50 & 0.346 & 0.362 & 0.381 & 0.403 & 0.458 & 18.2 & 18.6 & 19.4 & 20.4 & 19.3 \\
\recon & \M{3} & 5 & 0.341 & 0.358 & 0.377 & 0.401 & 0.459 & 21.8 & 22.4 & 23.3 & 24.2 & 23.2 \\
\recon & \M{4} & 50 & 0.345 & 0.361 & 0.379 & 0.402 & 0.457 & 17.9 & 18.1 & 19.1 & 20.0 & 19.1 \\
\recon & \M{4} & 5 & 0.340 & 0.356 & 0.375 & 0.400 & 0.458 & 21.5 & 21.9 & 22.9 & 23.9 & 22.9 \\
\recon & \mono & 50 & 0.341 & 0.356 & 0.374 & 0.396 & 0.452 & 18.0 & 18.1 & 18.9 & 19.3 & 18.4 \\
\recon & \mono & 5 & 0.335 & 0.350 & 0.369 & 0.394 & 0.453 & 20.7 & 21.2 & 21.7 & 22.7 & 21.8 \\
\recon & Standalone \M{1} & 50 & 0.348 & 0.363 & 0.381 & 0.404 & 0.458 & 19.3 & 19.7 & 20.3 & 20.7 & 20.2 \\
\recon & Standalone \M{1} & 5 & 0.344 & 0.359 & 0.378 & 0.402 & 0.460 & 22.7 & 23.3 & 23.9 & 24.7 & 23.8 \\
\recon & Standalone \M{0} & 50 & 0.368 & 0.383 & 0.399 & 0.420 & 0.472 & 19.9 & 20.4 & 21.3 & 22.3 & 21.2 \\
\recon & Standalone \M{0} & 5 & 0.366 & 0.380 & 0.397 & 0.419 & 0.471 & 23.9 & 24.7 & 26.2 & 27.2 & 26.3 \\
\midrule
\sacson & \M{1} & 50 & 0.332 & 0.339 & 0.343 & 0.348 & 0.379 & 18.8 & 18.9 & 19.1 & 19.4 & 21.0 \\
\sacson & \M{1} & 5 & 0.321 & 0.328 & 0.331 & 0.335 & 0.365 & 24.0 & 24.2 & 24.7 & 24.9 & 26.6 \\
\sacson & \M{2} & 50 & 0.329 & 0.336 & 0.340 & 0.345 & 0.375 & 17.9 & 18.0 & 18.2 & 18.6 & 20.1 \\
\sacson & \M{2} & 5 & 0.318 & 0.324 & 0.327 & 0.332 & 0.361 & 23.0 & 23.2 & 23.6 & 23.8 & 25.5 \\
\sacson & \M{3} & 50 & 0.326 & 0.333 & 0.336 & 0.341 & 0.371 & 17.1 & 17.2 & 17.6 & 17.9 & 19.2 \\
\sacson & \M{3} & 5 & 0.314 & 0.320 & 0.324 & 0.328 & 0.358 & 21.8 & 22.1 & 22.5 & 22.8 & 24.6 \\
\sacson & \M{4} & 50 & 0.323 & 0.330 & 0.333 & 0.338 & 0.369 & 16.8 & 16.9 & 17.1 & 17.5 & 18.7 \\
\sacson & \M{4} & 5 & 0.311 & 0.317 & 0.320 & 0.325 & 0.355 & 21.1 & 21.3 & 21.6 & 22.1 & 23.7 \\
\sacson & \mono & 50 & 0.314 & 0.319 & 0.323 & 0.328 & 0.361 & 16.1 & 16.4 & 16.5 & 16.8 & 17.8 \\
\sacson & \mono & 5 & 0.302 & 0.307 & 0.310 & 0.315 & 0.347 & 20.3 & 20.5 & 20.5 & 20.9 & 22.4 \\
\sacson & Standalone \M{1} & 50 & 0.325 & 0.331 & 0.334 & 0.340 & 0.371 & 17.2 & 17.4 & 17.7 & 17.9 & 19.5 \\
\sacson & Standalone \M{1} & 5 & 0.313 & 0.319 & 0.322 & 0.327 & 0.357 & 22.0 & 22.2 & 22.7 & 23.0 & 24.8 \\
\sacson & Standalone \M{0} & 50 & 0.349 & 0.355 & 0.358 & 0.364 & 0.392 & 20.5 & 21.1 & 20.9 & 21.5 & 23.4 \\
\sacson & Standalone \M{0} & 5 & 0.337 & 0.342 & 0.345 & 0.349 & 0.376 & 27.1 & 27.2 & 27.4 & 27.7 & 30.2 \\
\midrule
\scand & \M{1} & 50 & 0.349 & 0.373 & 0.399 & 0.428 & 0.459 & 27.1 & 28.5 & 31.1 & 33.0 & 35.6 \\
\scand & \M{1} & 5 & 0.337 & 0.362 & 0.389 & 0.419 & 0.452 & 30.9 & 33.8 & 36.4 & 39.4 & 41.4 \\
\scand & \M{2} & 50 & 0.349 & 0.373 & 0.399 & 0.427 & 0.458 & 26.5 & 28.0 & 30.5 & 32.3 & 34.4 \\
\scand & \M{2} & 5 & 0.336 & 0.361 & 0.389 & 0.419 & 0.451 & 30.0 & 32.9 & 35.4 & 37.5 & 39.4 \\
\scand & \M{3} & 50 & 0.348 & 0.373 & 0.399 & 0.427 & 0.458 & 25.9 & 27.6 & 29.6 & 31.3 & 33.2 \\
\scand & \M{3} & 5 & 0.336 & 0.361 & 0.389 & 0.418 & 0.450 & 29.4 & 31.9 & 34.4 & 36.7 & 38.0 \\
\scand & \M{4} & 50 & 0.349 & 0.373 & 0.399 & 0.427 & 0.458 & 25.6 & 27.2 & 29.1 & 31.1 & 32.8 \\
\scand & \M{4} & 5 & 0.336 & 0.362 & 0.389 & 0.418 & 0.450 & 29.0 & 31.3 & 34.1 & 36.3 & 37.3 \\
\scand & \mono & 50 & 0.362 & 0.384 & 0.405 & 0.428 & 0.456 & 26.7 & 27.9 & 28.5 & 29.9 & 31.3 \\
\scand & \mono & 5 & 0.352 & 0.375 & 0.397 & 0.421 & 0.450 & 30.4 & 31.8 & 33.3 & 34.7 & 35.5 \\
\scand & Standalone \M{1} & 50 & 0.352 & 0.376 & 0.401 & 0.426 & 0.456 & 26.8 & 28.3 & 30.1 & 32.3 & 34.2 \\
\scand & Standalone \M{1} & 5 & 0.340 & 0.365 & 0.392 & 0.419 & 0.450 & 30.6 & 33.0 & 35.8 & 38.2 & 39.4 \\
\scand & Standalone \M{0} & 50 & 0.364 & 0.384 & 0.408 & 0.435 & 0.467 & 30.4 & 31.9 & 33.6 & 35.4 & 38.4 \\
\scand & Standalone \M{0} & 5 & 0.351 & 0.372 & 0.398 & 0.427 & 0.461 & 35.3 & 37.9 & 41.1 & 43.7 & 45.8 \\
