# Supplementary material for: Fewer Steps, Better Plans: Sampling Variance in Flow-Matching Navigation World Models
Source: arXiv:2611.36153 source file (2026-11-26)
Supplement: Supplementary file 12 [file supp_kernel_bench_body.tex]

\mono & 13.18 / 12.02 & 480.6 & 196.2 & 6.70 & 213.5 & 87.2 & 4.71 & 2.25$\times$ \\
\M{4} & 15.04 / 14.04 & 482.2 & 196.9 & 6.70 & 214.7 & 87.7 & 4.71 & 2.25$\times$ \\
\M{3} & -- & 464.9 & 189.8 & 6.70 & 196.6 & 80.3 & 4.24 & 2.36$\times$ \\
\M{2} & -- & 456.1 & 186.2 & 6.70 & 187.2 & 76.5 & 4.24 & 2.44$\times$ \\
\M{1} & 14.48 / 15.40 & 451.6 & 184.4 & 6.70 & 182.4 & 74.5 & 4.24 & 2.48$\times$ \\
