# Supplementary material for: Fewer Steps, Better Plans: Sampling Variance in Flow-Matching Navigation World Models
Source: arXiv:2611.36153 source file (2026-11-26)
Supplement: Supplementary file 13 [file supp_noise_body.tex]

100 \sacson (seed 0) & \at{4}{50} & 5 & 0.87 & 0.77 & 0.88 & 0.52 & 2.82 & 2.71 & 2.65 & 2.63 \\
100 \sacson (seed 0) & \at{4}{5} & 3 & 0.61 & 0.58 & 0.61 & 0.69 & 2.76 & 2.63 & 2.60 & -- \\
100 \sacson (seed 0) & \at{1}{5} & 3 & 0.60 & 0.58 & 0.60 & 0.69 & 2.75 & 2.54 & 2.50 & -- \\
\midrule
500 \recon (seed 0) & \at{1}{50} & 3 & 0.67 & 0.65 & 0.67 & 0.65 & 1.379 & 1.341 & 1.341 & -- \\
500 \sacson (seed 0) & \at{1}{50} & 3 & 0.83 & 0.80 & 0.90 & 0.52 & 2.818 & 2.703 & 2.636 & -- \\
\midrule
500 \recon (seeds 0--2) & \at{1}{5} & 3 & 0.48 & 0.47 & 0.46 & 0.79 & 1.278 & 1.252 & 1.247 & -- \\
500 \sacson (seeds 0--2) & \at{1}{5} & 3 & 0.61 & 0.59 & 0.62 & 0.69 & 2.754 & 2.638 & 2.592 & -- \\
500 \scand (seeds 0--2) & \at{1}{5} & 3 & 0.42 & 0.41 & 0.37 & 0.82 & 1.004 & 1.001 & 0.998 & -- \\
\midrule
500 \recon (seeds 0--2) & \at{1}{3} & 2 & 0.32 & 0.32 & 0.30 & 0.88 & 1.256 & 1.240 & -- & -- \\
500 \sacson (seeds 0--2) & \at{1}{3} & 2 & 0.43 & 0.43 & 0.44 & 0.81 & 2.719 & 2.627 & -- & -- \\
500 \scand (seeds 0--2) & \at{1}{3} & 2 & 0.31 & 0.31 & 0.27 & 0.89 & 0.988 & 1.003 & -- & -- \\
500 \recon (seeds 0--2) & \at{4}{3} & 2 & 0.32 & 0.32 & 0.30 & 0.89 & 1.250 & 1.238 & -- & -- \\
500 \sacson (seeds 0--2) & \at{4}{3} & 2 & 0.43 & 0.43 & 0.45 & 0.81 & 2.738 & 2.644 & -- & -- \\
500 \scand (seeds 0--2) & \at{4}{3} & 2 & 0.31 & 0.31 & 0.28 & 0.88 & 1.002 & 0.994 & -- & -- \\
500 \recon (seeds 0--2) & \monoat{3} & 2 & 0.34 & 0.34 & 0.33 & 0.88 & 1.277 & 1.255 & -- & -- \\
500 \sacson (seeds 0--2) & \monoat{3} & 2 & 0.41 & 0.41 & 0.42 & 0.83 & 2.667 & 2.591 & -- & -- \\
500 \scand (seeds 0--2) & \monoat{3} & 2 & 0.33 & 0.33 & 0.28 & 0.87 & 1.050 & 1.051 & -- & -- \\
\midrule
500 \recon (seeds 0--2) & \at{1}{2} & 4 & 0.10 & 0.10 & 0.10 & 0.98 & 1.251 & 1.253 & 1.256 & 1.257 \\
500 \sacson (seeds 0--2) & \at{1}{2} & 4 & 0.23 & 0.22 & 0.25 & 0.94 & 2.792 & 2.769 & 2.759 & 2.756 \\
500 \scand (seeds 0--2) & \at{1}{2} & 4 & 0.10 & 0.10 & 0.09 & 0.98 & 1.000 & 1.002 & 1.000 & 0.998 \\
500 \recon (seeds 0--2) & \monoat{2} & 4 & 0.11 & 0.11 & 0.11 & 0.98 & 1.264 & 1.263 & 1.263 & 1.263 \\
500 \sacson (seeds 0--2) & \monoat{2} & 4 & 0.22 & 0.21 & 0.24 & 0.95 & 2.691 & 2.669 & 2.661 & 2.663 \\
500 \scand (seeds 0--2) & \monoat{2} & 4 & 0.11 & 0.11 & 0.09 & 0.98 & 1.090 & 1.092 & 1.088 & 1.088 \\
\midrule
\multicolumn{11}{@{}l}{\emph{Second-order solver noise-to-signal on the nested \paper \M{1} shard (100 items/dataset, shard 0/5, seed 0)}} \\
100 \recon (shard 0/5) & \at{1}{5} (Euler, 4 NFE) & 3 & 0.48 & 0.47 & 0.46 & 0.78 & 1.279 & 1.222 & 1.210 & -- \\
100 \recon (shard 0/5) & \at{1}{3} (Euler, 2 NFE) & 2 & 0.32 & 0.32 & 0.30 & 0.88 & 1.259 & 1.205 & -- & -- \\
100 \recon (shard 0/5) & \at{1}{3} (Heun, 4 NFE) & 3 & 0.46 & 0.45 & 0.44 & 0.81 & 1.402 & 1.422 & 1.366 & -- \\
100 \recon (shard 0/5) & \at{1}{3} (midpoint, 4 NFE) & 3 & 0.54 & 0.52 & 0.53 & 0.75 & 1.370 & 1.337 & 1.321 & -- \\
\midrule
100 \sacson (shard 0/5) & \at{1}{5} (Euler, 4 NFE) & 3 & 0.62 & 0.59 & 0.63 & 0.67 & 2.587 & 2.464 & 2.428 & -- \\
100 \sacson (shard 0/5) & \at{1}{3} (Euler, 2 NFE) & 2 & 0.44 & 0.44 & 0.46 & 0.79 & 2.587 & 2.550 & -- & -- \\
100 \sacson (shard 0/5) & \at{1}{3} (Heun, 4 NFE) & 3 & 0.49 & 0.47 & 0.47 & 0.76 & 2.731 & 2.712 & 2.685 & -- \\
100 \sacson (shard 0/5) & \at{1}{3} (midpoint, 4 NFE) & 3 & 0.60 & 0.58 & 0.59 & 0.68 & 2.696 & 2.551 & 2.484 & -- \\
\midrule
100 \scand (shard 0/5) & \at{1}{5} (Euler, 4 NFE) & 3 & 0.41 & 0.40 & 0.36 & 0.83 & 1.129 & 1.167 & 1.145 & -- \\
100 \scand (shard 0/5) & \at{1}{3} (Euler, 2 NFE) & 2 & 0.31 & 0.31 & 0.27 & 0.89 & 1.107 & 1.125 & -- & -- \\
100 \scand (shard 0/5) & \at{1}{3} (Heun, 4 NFE) & 3 & 0.37 & 0.36 & 0.30 & 0.85 & 1.148 & 1.136 & 1.111 & -- \\
100 \scand (shard 0/5) & \at{1}{3} (midpoint, 4 NFE) & 3 & 0.41 & 0.40 & 0.35 & 0.83 & 1.128 & 1.143 & 1.137 & -- \\
