# Supplementary material for: Fewer Steps, Better Plans: Sampling Variance in Flow-Matching Navigation World Models
Source: arXiv:2611.36153 source file (2026-11-26)
Supplement: Supplementary file 14 [file supp_nullcal_body.tex]

Same configuration, two seeds & 0 / 30 & 0.89 & 3 / 30 & 1.24 & 0 / 30 & 0.94 & 3 / 90 & 1.06 \\
Model difference, two seeds & 2 / 24 & 1.25 & 9 / 24 & 1.69 & 0 / 24 & 0.78 & 11 / 72 & 1.30 \\
Step-count difference, two seeds & 1 / 27 & 1.14 & 2 / 27 & 1.00 & 4 / 27 & 0.99 & 7 / 81 & 1.07 \\
\midrule
All & 3 / 81 & 1.08 & 14 / 81 & 1.36 & 4 / 81 & 1.04 & 21 / 243 & 1.17 \\
