# Supplementary material for: Fewer Steps, Better Plans: Sampling Variance in Flow-Matching Navigation World Models
Source: arXiv:2611.36153 source file (2026-11-26)
Supplement: Supplementary file 15 [file supp_plan_full_body.tex]

All-\M{1} & 50 & 1.37 & 0.366 & 2.78 & 0.683 & 1.01 & 0.284 & 176.1 \\
 & 20 & 1.34 & 0.365 & 2.79 & 0.688 & 1.02 & 0.283 & 68.6 \\
 & 10 & 1.32 & 0.365 & 2.74 & 0.684 & 0.99 & 0.280 & 32.8 \\
 & 5 & 1.26 & 0.364 & 2.68 & 0.681 & 1.00 & 0.282 & 14.9 \\
 & 4 & 1.27 & 0.369 & 2.67 & 0.683 & 1.00 & 0.282 & 11.2 \\
 & 3 & 1.24 & 0.370 & 2.67 & 0.688 & 1.01 & 0.284 & 7.6 \\
 & 2 & 1.26 & 0.379 & 2.80 & 0.708 & 0.99 & 0.281 & 4.0 \\
\midrule
All-\M{2} & 5 & 1.26 & 0.364 & 2.71 & 0.679 & 1.01 & 0.285 & 14.9 \\
\midrule
All-\M{3} & 5 & 1.27 & 0.361 & 2.75 & 0.685 & 1.00 & 0.280 & 15.2 \\
\midrule
All-\M{4} & 50 & 1.38 & 0.371 & 2.81 & 0.686 & 1.02 & 0.284 & 188.2 \\
 & 20 & 1.34 & 0.369 & 2.82 & 0.691 & 1.01 & 0.280 & 73.2 \\
 & 10 & 1.31 & 0.366 & 2.76 & 0.680 & 1.00 & 0.280 & 34.9 \\
 & 5 & 1.27 & 0.361 & 2.71 & 0.680 & 1.00 & 0.278 & 15.7 \\
 & 3 & 1.25 & 0.367 & 2.69 & 0.684 & 1.01 & 0.282 & 8.0 \\
 & 2 & 1.25 & 0.373 & 2.76 & 0.698 & 0.99 & 0.280 & 4.2 \\
\midrule
\mono & 50 & 1.35 & 0.366 & 2.85 & 0.696 & 1.01 & 0.286 & 187.6 \\
 & 20 & 1.35 & 0.367 & 2.85 & 0.695 & 1.03 & 0.289 & 73.0 \\
 & 10 & 1.32 & 0.364 & 2.80 & 0.689 & 1.00 & 0.285 & 34.9 \\
 & 5 & 1.29 & 0.363 & 2.78 & 0.687 & 1.01 & 0.284 & 15.7 \\
 & 4 & 1.29 & 0.368 & 2.72 & 0.681 & 1.04 & 0.288 & 11.9 \\
 & 3 & 1.27 & 0.367 & 2.73 & 0.690 & 1.07 & 0.293 & 8.0 \\
 & 2 & 1.26 & 0.367 & 2.71 & 0.685 & 1.10 & 0.299 & 4.2 \\
\midrule
\mono, naive \M{1} slice & 5 & 1.73 & 0.487 & 4.86 & 1.068 & 1.09 & 0.307 & 14.8 \\
