# Supplementary material for: Fewer Steps, Better Plans: Sampling Variance in Flow-Matching Navigation World Models
Source: arXiv:2611.36153 source file (2026-11-26)
Supplement: Supplementary file 16 [file supp_pooled_body.tex]

\multicolumn{7}{@{}l}{\emph{Granularity at a fixed step count}} \\
\M{1}@50 $-$ {\mono}@50 & $+0.020$ / $+0.022$ / $-0.028$ & $+0.005$ [$-0.021$, $+0.032$] & $-0.070$ / $+0.085$ / $-0.020$ & $-0.002$ [$-0.064$, $+0.053$] & $+0.002$ / $-0.027$ / $-0.012$ & $-0.012$ [$-0.036$, $+0.013$] \\
\M{1}@5 $-$ {\mono}@5 & $-0.035$ / $-0.054$\sig / $+0.002$ & $-0.029$\sig [$-0.054$, $-0.004$] & $-0.101$\sig / $+0.113$\sig / $-0.036$ & $-0.008$ [$-0.065$, $+0.052$] & $-0.007$ / $-0.030$ / $-0.026$ & $-0.021$ [$-0.044$, $+0.003$] \\
\M{1}@3 $-$ {\mono}@3 & $-0.028$ / $-0.038$ / $-0.006$ & $-0.024$ [$-0.049$, $+0.001$] & $-0.056$ / $+0.123$\sig / $+0.090$\sig & $+0.053$ [$-0.009$, $+0.113$] & $-0.061$\sig / $-0.077$\sig / $-0.043$\sig & $-0.060$\sig [$-0.090$, $-0.033$] \\
\M{1}@2 $-$ {\mono}@2 & $-0.002$ / $-0.027$ / $-0.017$ & $-0.015$ [$-0.044$, $+0.016$] & $+0.097$ / $+0.118$\sig / $+0.092$ & $+0.102$\sig [$+0.032$, $+0.175$] & $-0.110$\sig / $-0.088$\sig / $-0.096$\sig & $-0.098$\sig [$-0.128$, $-0.069$] \\
\M{4}@50 $-$ {\mono}@50 & $+0.025$ / $+0.007$ / $-0.025$ & $+0.002$ [$-0.023$, $+0.028$] & $-0.042$ / $+0.067$ / $-0.046$ & $-0.007$ [$-0.064$, $+0.053$] & $+0.012$ / $-0.049$\sig / $+0.009$ & $-0.009$ [$-0.033$, $+0.013$] \\
\M{4}@5 $-$ {\mono}@5 & $-0.024$ / $-0.016$ / $-0.031$ & $-0.024$ [$-0.048$, $+0.001$] & $-0.065$ / $+0.077$ / $+0.033$ & $+0.015$ [$-0.038$, $+0.071$] & $-0.010$ / $-0.041$ / $-0.028$ & $-0.027$\sig [$-0.051$, $-0.002$] \\
\M{4}@3 $-$ {\mono}@3 & $-0.021$ / $-0.038$\sig / $-0.004$ & $-0.021$ [$-0.045$, $+0.004$] & $-0.037$ / $+0.142$\sig / $+0.132$\sig & $+0.079$\sig [$+0.018$, $+0.142$] & $-0.068$\sig / $-0.062$\sig / $-0.021$ & $-0.050$\sig [$-0.081$, $-0.021$] \\
\M{4}@2 $-$ {\mono}@2 & $-0.015$ / $-0.018$ / $-0.030$ & $-0.021$ [$-0.049$, $+0.007$] & $+0.056$ / $+0.076$ / $+0.011$ & $+0.048$ [$-0.027$, $+0.120$] & $-0.104$\sig / $-0.088$\sig / $-0.095$\sig & $-0.096$\sig [$-0.124$, $-0.067$] \\
\M{1}@50 $-$ \M{4}@50 & $-0.005$ / $+0.015$ / $-0.002$ & $+0.003$ [$-0.019$, $+0.024$] & $-0.028$ / $+0.018$ / $+0.026$ & $+0.005$ [$-0.045$, $+0.051$] & $-0.010$ / $+0.022$ / $-0.021$ & $-0.003$ [$-0.023$, $+0.018$] \\
\M{1}@5 $-$ \M{4}@5 & $-0.011$ / $-0.038$\sig / $+0.033$\sig & $-0.005$ [$-0.025$, $+0.013$] & $-0.036$ / $+0.036$ / $-0.069$ & $-0.023$ [$-0.067$, $+0.021$] & $+0.003$ / $+0.011$ / $+0.002$ & $+0.006$ [$-0.016$, $+0.025$] \\
\M{1}@3 $-$ \M{4}@3 & $-0.007$ / $+0.000$ / $-0.002$ & $-0.003$ [$-0.020$, $+0.013$] & $-0.019$ / $-0.019$ / $-0.042$ & $-0.027$ [$-0.072$, $+0.015$] & $+0.007$ / $-0.014$ / $-0.023$ & $-0.010$ [$-0.029$, $+0.010$] \\
\M{1}@2 $-$ \M{4}@2 & $+0.013$ / $-0.009$ / $+0.013$ & $+0.006$ [$-0.013$, $+0.023$] & $+0.041$ / $+0.042$ / $+0.081$\sig & $+0.055$\sig [$+0.011$, $+0.099$] & $-0.006$ / $0.000$ / $-0.001$ & $-0.002$ [$-0.022$, $+0.017$] \\
Standalone \M{1}@50 $-$ \M{1}@50 & $-0.015$ / $-0.011$ / $+0.028$ & $+0.001$ [$-0.024$, $+0.026$] & $+0.048$ / $-0.070$ / $-0.003$ & $-0.008$ [$-0.058$, $+0.049$] & $-0.009$ / $-0.007$ / $+0.004$ & $-0.004$ [$-0.026$, $+0.019$] \\
Standalone \M{1}@50 $-$ {\mono}@50 & $+0.005$ / $+0.011$ / $+0.001$ & $+0.006$ [$-0.020$, $+0.034$] & $-0.022$ / $+0.014$ / $-0.022$ & $-0.010$ [$-0.062$, $+0.052$] & $-0.007$ / $-0.033$ / $-0.008$ & $-0.016$ [$-0.038$, $+0.006$] \\
Standalone \M{1}@5 $-$ \M{1}@5 & $+0.026$ / $+0.032$ / $-0.017$ & $+0.013$ [$-0.009$, $+0.036$] & $+0.017$ / $-0.100$\sig / $-0.012$ & $-0.032$ [$-0.085$, $+0.025$] & $-0.016$ / $-0.011$ / $-0.023$ & $-0.017$ [$-0.039$, $+0.005$] \\
Standalone \M{1}@5 $-$ {\mono}@5 & $-0.009$ / $-0.022$ / $-0.015$ & $-0.016$ [$-0.040$, $+0.008$] & $-0.083$ / $+0.012$ / $-0.047$ & $-0.040$ [$-0.098$, $+0.021$] & $-0.023$ / $-0.042$ / $-0.048$\sig & $-0.038$\sig [$-0.063$, $-0.011$] \\
Standalone \M{0}@50 $-$ \M{1}@5 & $+0.160$\sig / $+0.152$\sig / $+0.095$\sig & $+0.136$\sig [$+0.106$, $+0.171$] & $+0.333$\sig / $+0.173$\sig / $+0.306$\sig & $+0.271$\sig [$+0.198$, $+0.340$] & $+0.010$ / $+0.009$ / $+0.024$ & $+0.014$ [$-0.009$, $+0.040$] \\
Standalone \M{0}@5 $-$ \M{1}@5 & $+0.011$ / $+0.004$ / $-0.022$ & $-0.002$ [$-0.029$, $+0.026$] & $+0.189$\sig / $+0.084$ / $+0.231$\sig & $+0.168$\sig [$+0.094$, $+0.241$] & $-0.014$ / $+0.010$ / $-0.006$ & $-0.003$ [$-0.028$, $+0.022$] \\
Standalone \M{0}@3 $-$ \M{1}@5 & $+0.009$ / $+0.006$ / $+0.026$ & $+0.014$ [$-0.017$, $+0.042$] & $+0.194$\sig / $+0.085$ / $+0.198$\sig & $+0.159$\sig [$+0.084$, $+0.233$] & $-0.007$ / $+0.016$ / $-0.024$ & $-0.005$ [$-0.032$, $+0.021$] \\
Standalone \M{0}@2 $-$ \M{1}@2 & $+0.014$ / $+0.049$\sig / $+0.046$\sig & $+0.037$\sig [$+0.008$, $+0.066$] & $+0.105$ / $+0.141$\sig / $+0.081$ & $+0.109$\sig [$+0.022$, $+0.192$] & $+0.030$ / $+0.037$ / $-0.015$ & $+0.017$ [$-0.010$, $+0.046$] \\
\midrule
\multicolumn{7}{@{}l}{\emph{Against the 50-step monolithic protocol}} \\
\M{1}@5 $-$ {\mono}@50 & $-0.092$\sig / $-0.112$\sig / $-0.085$\sig & $-0.096$\sig [$-0.126$, $-0.068$] & $-0.171$\sig / $+0.020$ / $-0.115$\sig & $-0.089$\sig [$-0.148$, $-0.028$] & $-0.011$ / $-0.043$\sig / $-0.027$ & $-0.027$\sig [$-0.051$, $-0.004$] \\
\M{1}@3 $-$ {\mono}@50 & $-0.108$\sig / $-0.117$\sig / $-0.122$\sig & $-0.116$\sig [$-0.149$, $-0.084$] & $-0.174$\sig / $-0.070$ / $-0.125$\sig & $-0.123$\sig [$-0.185$, $-0.053$] & $+0.002$ / $-0.075$\sig / $-0.048$\sig & $-0.040$\sig [$-0.067$, $-0.014$] \\
\M{1}@2 $-$ {\mono}@50 & $-0.090$\sig / $-0.126$\sig / $-0.124$\sig & $-0.114$\sig [$-0.152$, $-0.074$] & $-0.045$ / $-0.021$ / $-0.015$ & $-0.027$ [$-0.104$, $+0.057$] & $-0.023$ / $-0.057$\sig / $-0.043$ & $-0.041$\sig [$-0.071$, $-0.012$] \\
{\mono}@5 $-$ {\mono}@50 & $-0.057$\sig / $-0.058$\sig / $-0.087$\sig & $-0.067$\sig [$-0.091$, $-0.043$] & $-0.070$ / $-0.093$\sig / $-0.080$\sig & $-0.081$\sig [$-0.126$, $-0.033$] & $-0.004$ / $-0.013$ / $-0.002$ & $-0.006$ [$-0.027$, $+0.014$] \\
{\mono}@3 $-$ {\mono}@50 & $-0.080$\sig / $-0.079$\sig / $-0.116$\sig & $-0.092$\sig [$-0.121$, $-0.063$] & $-0.118$\sig / $-0.193$\sig / $-0.216$\sig & $-0.176$\sig [$-0.233$, $-0.110$] & $+0.063$\sig / $+0.002$ / $-0.005$ & $+0.020$ [$-0.006$, $+0.045$] \\
Standalone \M{0}@50 $-$ {\mono}@50 & $+0.068$\sig / $+0.040$ / $+0.010$ & $+0.039$\sig [$+0.009$, $+0.072$] & $+0.162$\sig / $+0.192$\sig / $+0.190$\sig & $+0.182$\sig [$+0.115$, $+0.250$] & $-0.002$ / $-0.034$ / $-0.003$ & $-0.013$ [$-0.038$, $+0.011$] \\
Standalone \M{0}@5 $-$ {\mono}@50 & $-0.081$\sig / $-0.108$\sig / $-0.107$\sig & $-0.099$\sig [$-0.132$, $-0.064$] & $+0.018$ / $+0.104$ / $+0.116$ & $+0.079$\sig [$+0.000$, $+0.154$] & $-0.025$ / $-0.032$ / $-0.033$ & $-0.030$\sig [$-0.055$, $-0.007$] \\
\midrule
\multicolumn{7}{@{}l}{\emph{Step count within a model}} \\
\M{1}@5 $-$ \M{1}@50 & $-0.112$\sig / $-0.134$\sig / $-0.058$\sig & $-0.101$\sig [$-0.127$, $-0.077$] & $-0.101$\sig / $-0.065$ / $-0.096$\sig & $-0.087$\sig [$-0.133$, $-0.037$] & $-0.014$ / $-0.016$ / $-0.015$ & $-0.015$ [$-0.038$, $+0.007$] \\
\M{1}@3 $-$ \M{1}@5 & $-0.016$ / $-0.005$ / $-0.036$\sig & $-0.019$\sig [$-0.040$, $-0.001$] & $-0.003$ / $-0.089$\sig / $-0.010$ & $-0.034$ [$-0.079$, $+0.018$] & $+0.013$ / $-0.032$ / $-0.021$ & $-0.013$ [$-0.034$, $+0.008$] \\
\M{1}@2 $-$ \M{1}@5 & $+0.002$ / $-0.014$ / $-0.039$ & $-0.017$ [$-0.044$, $+0.011$] & $+0.126$\sig / $-0.040$ / $+0.101$\sig & $+0.062$ [$-0.004$, $+0.135$] & $-0.012$ / $-0.014$ / $-0.016$ & $-0.014$ [$-0.041$, $+0.013$] \\
\M{4}@5 $-$ \M{4}@50 & $-0.106$\sig / $-0.081$\sig / $-0.093$\sig & $-0.093$\sig [$-0.119$, $-0.071$] & $-0.094$\sig / $-0.083$ / $-0.001$ & $-0.059$\sig [$-0.107$, $-0.009$] & $-0.027$ / $-0.005$ / $-0.038$\sig & $-0.023$\sig [$-0.043$, $-0.002$] \\
\M{4}@2 $-$ \M{4}@5 & $-0.022$ / $-0.043$\sig / $-0.019$ & $-0.028$ [$-0.058$, $+0.001$] & $+0.049$ / $-0.046$ / $-0.049$ & $-0.015$ [$-0.085$, $+0.057$] & $-0.003$ / $-0.003$ / $-0.013$ & $-0.006$ [$-0.034$, $+0.021$] \\
\M{4}@2 $-$ \M{4}@50 & $-0.128$\sig / $-0.124$\sig / $-0.112$\sig & $-0.121$\sig [$-0.158$, $-0.087$] & $-0.044$ / $-0.129$\sig / $-0.050$ & $-0.074$\sig [$-0.150$, $-0.006$] & $-0.029$ / $-0.008$ / $-0.051$\sig & $-0.030$\sig [$-0.059$, $-0.002$] \\
Standalone \M{1}@5 $-$ Standalone \M{1}@50 & $-0.071$\sig / $-0.091$\sig / $-0.103$\sig & $-0.089$\sig [$-0.114$, $-0.065$] & $-0.132$\sig / $-0.095$\sig / $-0.105$\sig & $-0.111$\sig [$-0.156$, $-0.063$] & $-0.020$ / $-0.021$ / $-0.042$\sig & $-0.028$\sig [$-0.050$, $-0.008$] \\
Standalone \M{0}@5 $-$ Standalone \M{0}@50 & $-0.149$\sig / $-0.148$\sig / $-0.117$\sig & $-0.138$\sig [$-0.169$, $-0.110$] & $-0.144$\sig / $-0.088$ / $-0.075$ & $-0.102$\sig [$-0.160$, $-0.049$] & $-0.024$ / $+0.002$ / $-0.030$ & $-0.017$ [$-0.038$, $+0.006$] \\
{\mono}@3 $-$ {\mono}@5 & $-0.023$ / $-0.021$ / $-0.029$ & $-0.024$\sig [$-0.045$, $-0.004$] & $-0.048$ / $-0.100$\sig / $-0.136$\sig & $-0.094$\sig [$-0.135$, $-0.050$] & $+0.067$\sig / $+0.014$ / $-0.003$ & $+0.026$\sig [$+0.007$, $+0.046$] \\
{\mono}@2 $-$ {\mono}@5 & $-0.031$ / $-0.041$\sig / $-0.020$ & $-0.031$\sig [$-0.063$, $-0.003$] & $-0.072$ / $-0.046$ / $-0.027$ & $-0.048$ [$-0.108$, $+0.022$] & $+0.091$\sig / $+0.043$\sig / $+0.054$\sig & $+0.063$\sig [$+0.031$, $+0.092$] \\
\midrule
\multicolumn{7}{@{}l}{\emph{Second-order solvers at matched compute ($S{=}3$, 4 evaluations per frame)}} \\
\M{1}@3, Heun $-$ \M{1}@5 & $+0.146$\sig / $+0.155$\sig / $+0.122$\sig & $+0.141$\sig [$+0.111$, $+0.173$] & $+0.120$\sig / $-0.001$ / $+0.033$ & $+0.051$\sig [$+0.003$, $+0.101$] & $-0.007$ / $-0.001$ / $+0.007$ & $0.000$ [$-0.024$, $+0.022$] \\
\M{1}@3, midpoint $-$ \M{1}@5 & $+0.108$\sig / $+0.121$\sig / $+0.072$\sig & $+0.101$\sig [$+0.076$, $+0.126$] & $+0.105$\sig / $+0.019$ / $+0.009$ & $+0.044$\sig [$+0.001$, $+0.090$] & $+0.015$ / $+0.028$ / $+0.021$ & $+0.021$ [$-0.002$, $+0.045$] \\
{\mono}@3, Heun $-$ {\mono}@5 & $+0.088$\sig / $+0.078$\sig / $+0.106$\sig & $+0.091$\sig [$+0.063$, $+0.118$] & $+0.049$ / $+0.081$\sig / $+0.040$ & $+0.057$\sig [$+0.014$, $+0.104$] & $+0.038$\sig / $+0.026$ / $+0.007$ & $+0.024$\sig [$+0.003$, $+0.045$] \\
{\mono}@3, midpoint $-$ {\mono}@5 & $+0.092$\sig / $+0.070$\sig / $+0.081$\sig & $+0.081$\sig [$+0.057$, $+0.105$] & $+0.002$ / $-0.016$ / $-0.002$ & $-0.005$ [$-0.050$, $+0.036$] & $+0.022$ / $-0.007$ / $+0.009$ & $+0.008$ [$-0.013$, $+0.027$] \\
\M{1}@3, Heun $-$ \M{1}@50 & $+0.034$ / $+0.020$ / $+0.065$\sig & $+0.040$\sig [$+0.013$, $+0.069$] & $+0.019$ / $-0.066$ / $-0.063$ & $-0.037$ [$-0.087$, $+0.014$] & $-0.021$ / $-0.018$ / $-0.008$ & $-0.016$ [$-0.038$, $+0.006$] \\
\M{1}@3, midpoint $-$ \M{1}@50 & $-0.004$ / $-0.013$ / $+0.014$ & $-0.001$ [$-0.021$, $+0.021$] & $+0.003$ / $-0.046$ / $-0.087$\sig & $-0.043$ [$-0.084$, $+0.004$] & $+0.001$ / $+0.012$ / $+0.006$ & $+0.006$ [$-0.013$, $+0.024$] \\
{\mono}@3, Heun $-$ {\mono}@50 & $+0.031$ / $+0.020$ / $+0.019$ & $+0.023$ [$-0.004$, $+0.050$] & $-0.021$ / $-0.012$ / $-0.040$ & $-0.025$ [$-0.076$, $+0.032$] & $+0.034$ / $+0.013$ / $+0.006$ & $+0.018$ [$-0.004$, $+0.040$] \\
{\mono}@3, midpoint $-$ {\mono}@50 & $+0.035$\sig / $+0.013$ / $-0.006$ & $+0.014$ [$-0.006$, $+0.036$] & $-0.068$ / $-0.109$\sig / $-0.082$\sig & $-0.087$\sig [$-0.128$, $-0.040$] & $+0.018$ / $-0.020$ / $+0.007$ & $+0.002$ [$-0.015$, $+0.019$] \\
\M{1}@3, midpoint $-$ \M{1}@3, Heun & $-0.038$ / $-0.033$ / $-0.051$\sig & $-0.041$\sig [$-0.068$, $-0.014$] & $-0.016$ / $+0.020$ / $-0.024$ & $-0.007$ [$-0.051$, $+0.038$] & $+0.022$ / $+0.030$ / $+0.013$ & $+0.022$\sig [$+0.004$, $+0.042$] \\
{\mono}@3, midpoint $-$ {\mono}@3, Heun & $+0.004$ / $-0.008$ / $-0.025$ & $-0.009$ [$-0.034$, $+0.015$] & $-0.047$ / $-0.097$\sig / $-0.043$ & $-0.062$\sig [$-0.106$, $-0.020$] & $-0.016$ / $-0.033$ / $+0.001$ & $-0.016$ [$-0.036$, $+0.004$] \\
\midrule
\multicolumn{7}{@{}l}{\emph{Uniform-grid second-order solvers ($\alpha{=}1$, 4 evaluations per frame)}} \\
\M{1} unif.\ Heun $-$ \M{1}@5 & $+0.074$\sig / $+0.087$\sig / $+0.050$\sig & $+0.071$\sig [$+0.043$, $+0.102$] & $+0.070$ / $-0.053$ / $-0.005$ & $+0.004$ [$-0.061$, $+0.072$] & $+0.010$ / $+0.005$ / $+0.025$ & $+0.014$ [$-0.010$, $+0.039$] \\
\M{1} unif.\ midpoint $-$ \M{1}@5 & $+0.101$\sig / $+0.146$\sig / $+0.078$\sig & $+0.108$\sig [$+0.082$, $+0.136$] & $+0.074$ / $-0.042$ / $-0.044$ & $-0.004$ [$-0.060$, $+0.051$] & $+0.011$ / $+0.000$ / $+0.039$ & $+0.017$ [$-0.008$, $+0.042$] \\
{\mono} unif.\ Heun $-$ {\mono}@5 & $+0.050$\sig / $+0.051$\sig / $+0.072$\sig & $+0.058$\sig [$+0.029$, $+0.086$] & $-0.044$ / $-0.016$ / $-0.067$ & $-0.042$ [$-0.093$, $+0.015$] & $+0.001$ / $+0.012$ / $+0.012$ & $+0.008$ [$-0.016$, $+0.033$] \\
{\mono} unif.\ midpoint $-$ {\mono}@5 & $+0.072$\sig / $+0.091$\sig / $+0.108$\sig & $+0.090$\sig [$+0.062$, $+0.121$] & $+0.017$ / $-0.040$ / $-0.062$ & $-0.028$ [$-0.079$, $+0.023$] & $+0.033$ / $+0.000$ / $+0.015$ & $+0.016$ [$-0.005$, $+0.038$] \\
\M{1} unif.\ Heun $-$ \M{1}@3, Heun & $-0.072$\sig / $-0.067$\sig / $-0.072$\sig & $-0.071$\sig [$-0.101$, $-0.040$] & $-0.050$ / $-0.052$ / $-0.038$ & $-0.047$ [$-0.100$, $+0.008$] & $+0.018$ / $+0.007$ / $+0.018$ & $+0.014$ [$-0.008$, $+0.035$] \\
\M{1} unif.\ midpoint $-$ \M{1}@3, midpoint & $-0.007$ / $+0.024$ / $+0.006$ & $+0.008$ [$-0.019$, $+0.033$] & $-0.031$ / $-0.061$ / $-0.053$ & $-0.048$ [$-0.097$, $+0.007$] & $-0.003$ / $-0.028$ / $+0.018$ & $-0.004$ [$-0.025$, $+0.017$] \\
{\mono} unif.\ Heun $-$ {\mono}@3, Heun & $-0.039$ / $-0.027$ / $-0.034$ & $-0.033$\sig [$-0.062$, $-0.004$] & $-0.092$\sig / $-0.096$\sig / $-0.108$\sig & $-0.099$\sig [$-0.151$, $-0.045$] & $-0.037$ / $-0.014$ / $+0.005$ & $-0.015$ [$-0.037$, $+0.007$] \\
{\mono} unif.\ midpoint $-$ {\mono}@3, midpoint & $-0.020$ / $+0.021$ / $+0.026$ & $+0.009$ [$-0.016$, $+0.041$] & $+0.015$ / $-0.024$ / $-0.060$ & $-0.023$ [$-0.074$, $+0.031$] & $+0.011$ / $+0.008$ / $+0.006$ & $+0.008$ [$-0.013$, $+0.030$] \\
\midrule
\multicolumn{7}{@{}l}{\emph{Symmetric multi-draw score averaging ($3{,}840\text{--}11{,}520$ evaluations per decision)}} \\
\M{1}@3 (2 draws) $-$ {\mono}@3 (2 draws) & $-0.024$ / $-0.034$ / $+0.014$ & $-0.015$ [$-0.043$, $+0.012$] & $+0.001$ / $+0.108$\sig / $-0.001$ & $+0.036$ [$-0.027$, $+0.097$] & $-0.055$\sig / $-0.073$\sig / $-0.015$ & $-0.048$\sig [$-0.077$, $-0.021$] \\
\M{4}@3 (2 draws) $-$ {\mono}@3 (2 draws) & $-0.008$ / $-0.029$ / $-0.014$ & $-0.017$ [$-0.044$, $+0.008$] & $+0.064$ / $+0.066$ / $+0.028$ & $+0.053$ [$-0.012$, $+0.114$] & $-0.054$\sig / $-0.080$\sig / $-0.038$ & $-0.057$\sig [$-0.083$, $-0.030$] \\
\M{1}@3 (2 draws) $-$ \M{4}@3 (2 draws) & $-0.015$ / $-0.005$ / $+0.027$ & $+0.002$ [$-0.015$, $+0.021$] & $-0.063$\sig / $+0.042$ / $-0.029$ & $-0.017$ [$-0.053$, $+0.026$] & $-0.001$ / $+0.007$ / $+0.023$ & $+0.010$ [$-0.010$, $+0.029$] \\
\M{1}@2 (4 draws) $-$ {\mono}@2 (4 draws) & $+0.001$ / $-0.006$ / $-0.013$ & $-0.006$ [$-0.039$, $+0.027$] & $+0.112$\sig / $+0.093$ / $+0.076$ & $+0.094$\sig [$+0.023$, $+0.171$] & $-0.082$\sig / $-0.114$\sig / $-0.071$\sig & $-0.089$\sig [$-0.120$, $-0.058$] \\
\M{1}@3 (2 draws) $-$ \M{1}@5 & $-0.024$ / $-0.016$ / $-0.039$\sig & $-0.026$\sig [$-0.050$, $-0.004$] & $-0.064$ / $-0.167$\sig / $-0.134$\sig & $-0.122$\sig [$-0.171$, $-0.070$] & $+0.005$ / $-0.034$ / $+0.008$ & $-0.007$ [$-0.030$, $+0.016$] \\
\M{1}@3 (2 draws) $-$ \M{1}@3 & $-0.007$ / $-0.011$ / $-0.002$ & $-0.007$ [$-0.021$, $+0.009$] & $-0.062$\sig / $-0.077$\sig / $-0.124$\sig & $-0.088$\sig [$-0.121$, $-0.054$] & $-0.008$ / $-0.002$ / $+0.029$ & $+0.006$ [$-0.012$, $+0.024$] \\
\M{1}@3 (2 draws) $-$ \M{1}@2 (4 draws) & $-0.027$ / $-0.017$ / $-0.006$ & $-0.016$ [$-0.038$, $+0.004$] & $-0.157$\sig / $-0.072$ / $-0.159$\sig & $-0.130$\sig [$-0.192$, $-0.066$] & $+0.005$ / $-0.004$ / $+0.014$ & $+0.005$ [$-0.017$, $+0.028$] \\
{\mono}@3 (2 draws) $-$ {\mono}@5 & $-0.035$ / $-0.036$ / $-0.050$\sig & $-0.040$\sig [$-0.063$, $-0.018$] & $-0.166$\sig / $-0.162$\sig / $-0.168$\sig & $-0.165$\sig [$-0.213$, $-0.117$] & $+0.053$\sig / $+0.008$ / $-0.003$ & $+0.020$ [$-0.004$, $+0.043$] \\
{\mono}@3 (2 draws) $-$ {\mono}@3 & $-0.012$ / $-0.015$ / $-0.022$ & $-0.016$\sig [$-0.030$, $-0.002$] & $-0.118$\sig / $-0.062$\sig / $-0.032$ & $-0.071$\sig [$-0.106$, $-0.037$] & $-0.014$ / $-0.006$ / $0.000$ & $-0.007$ [$-0.025$, $+0.010$] \\
{\mono}@3 (2 draws) $-$ {\mono}@50 & $-0.092$\sig / $-0.094$\sig / $-0.137$\sig & $-0.108$\sig [$-0.137$, $-0.077$] & $-0.236$\sig / $-0.255$\sig / $-0.248$\sig & $-0.247$\sig [$-0.309$, $-0.181$] & $+0.049$\sig / $-0.004$ / $-0.004$ & $+0.013$ [$-0.012$, $+0.039$] \\
{\mono}@3 (2 draws) $-$ {\mono}@2 (4 draws) & $-0.003$ / $+0.012$ / $-0.032$ & $-0.008$ [$-0.033$, $+0.017$] & $-0.046$ / $-0.087$ / $-0.082$ & $-0.072$\sig [$-0.130$, $-0.012$] & $-0.022$ / $-0.045$\sig / $-0.042$\sig & $-0.036$\sig [$-0.059$, $-0.013$] \\
{\mono}@2 (4 draws) $-$ {\mono}@5 & $-0.032$ / $-0.048$\sig / $-0.018$ & $-0.033$\sig [$-0.064$, $-0.003$] & $-0.120$\sig / $-0.075$ / $-0.086$ & $-0.094$\sig [$-0.158$, $-0.024$] & $+0.075$\sig / $+0.053$\sig / $+0.040$ & $+0.056$\sig [$+0.026$, $+0.085$] \\
\M{4}@3 (2 draws) $-$ \M{4}@5 & $-0.019$ / $-0.049$\sig / $-0.033$ & $-0.034$\sig [$-0.059$, $-0.007$] & $-0.037$ / $-0.173$\sig / $-0.174$\sig & $-0.128$\sig [$-0.175$, $-0.076$] & $+0.009$ / $-0.030$ / $-0.013$ & $-0.011$ [$-0.035$, $+0.012$] \\
\M{4}@3 (2 draws) $-$ \M{4}@50 & $-0.125$\sig / $-0.130$\sig / $-0.126$\sig & $-0.127$\sig [$-0.162$, $-0.095$] & $-0.130$\sig / $-0.256$\sig / $-0.175$\sig & $-0.187$\sig [$-0.243$, $-0.128$] & $-0.017$ / $-0.035$ / $-0.051$\sig & $-0.034$\sig [$-0.061$, $-0.010$] \\
\M{1}@5 (3 draws) $-$ \M{1}@50 & $-0.124$\sig / $-0.130$\sig / $-0.107$\sig & $-0.120$\sig [$-0.147$, $-0.093$] & $-0.177$\sig / $-0.276$\sig / $-0.279$\sig & $-0.244$\sig [$-0.298$, $-0.185$] & $-0.008$ / $-0.053$\sig / $-0.022$ & $-0.027$\sig [$-0.053$, $-0.004$] \\
\M{1}@3 (2 draws) $-$ \M{1}@5 (3 draws) & $-0.012$ / $-0.020$ / $+0.011$ & $-0.007$ [$-0.029$, $+0.014$] & $+0.011$ / $+0.044$ / $+0.049$ & $+0.035$ [$-0.011$, $+0.079$] & $-0.001$ / $+0.002$ / $+0.014$ & $+0.005$ [$-0.017$, $+0.028$] \\
\midrule
5\,\% margin & \multicolumn{2}{c}{0.068} & \multicolumn{2}{c}{0.142} & \multicolumn{2}{c}{0.052} \\
