# Supplementary material for: Fewer Steps, Better Plans: Sampling Variance in Flow-Matching Navigation World Models
Source: arXiv:2611.36153 source file (2026-11-26)
Supplement: Supplementary file 17 [file supp_r4_r5_ci_body.tex]

\multicolumn{4}{@{}l}{\emph{Symmetric two-draw score averaging at three steps ($S{=}3$, $3{,}840$ evaluations, seeds 0--2)}} \\
2 draws \at{1}{3} ($3{,}840$) $-$ 2 draws \monoat{3} ($3{,}840$) & $-0.015$ [$-0.043$, $+0.012$] & $+0.036$ [$-0.027$, $+0.097$] & $-0.048$\sig [$-0.077$, $-0.021$] \\
2 draws \at{4}{3} ($3{,}840$) $-$ 2 draws \monoat{3} ($3{,}840$) & $-0.017$ [$-0.044$, $+0.008$] & $+0.053$ [$-0.012$, $+0.114$] & $-0.057$\sig [$-0.083$, $-0.030$] \\
2 draws \at{1}{3} ($3{,}840$) $-$ 1 draw \at{1}{5} ($3{,}840$) & $-0.026$\sig [$-0.050$, $-0.004$] & $-0.122$\sig [$-0.171$, $-0.070$] & $-0.007$ [$-0.030$, $+0.016$] \\
2 draws \at{1}{3} ($3{,}840$) $-$ 1 draw \at{1}{3} ($1{,}920$) & $-0.007$ [$-0.021$, $+0.009$] & $-0.088$\sig [$-0.121$, $-0.054$] & $+0.006$ [$-0.012$, $+0.024$] \\
2 draws \at{1}{3} ($3{,}840$) $-$ 1 draw \at{1}{50} ($47{,}040$) & $-0.127$\sig [$-0.159$, $-0.096$] & $-0.209$\sig [$-0.268$, $-0.147$] & $-0.022$ [$-0.053$, $+0.005$] \\
2 draws \monoat{3} ($3{,}840$) $-$ 1 draw \monoat{5} ($3{,}840$) & $-0.040$\sig [$-0.063$, $-0.018$] & $-0.165$\sig [$-0.213$, $-0.117$] & $+0.020$ [$-0.004$, $+0.043$] \\
2 draws \monoat{3} ($3{,}840$) $-$ 1 draw \monoat{3} ($1{,}920$) & $-0.016$\sig [$-0.030$, $-0.002$] & $-0.071$\sig [$-0.106$, $-0.037$] & $-0.007$ [$-0.025$, $+0.010$] \\
2 draws \monoat{3} ($3{,}840$) $-$ 1 draw \monoat{50} ($47{,}040$) & $-0.108$\sig [$-0.137$, $-0.077$] & $-0.247$\sig [$-0.309$, $-0.181$] & $+0.013$ [$-0.012$, $+0.039$] \\
2 draws \at{4}{3} ($3{,}840$) $-$ 1 draw \at{4}{5} ($3{,}840$) & $-0.034$\sig [$-0.059$, $-0.007$] & $-0.128$\sig [$-0.175$, $-0.076$] & $-0.011$ [$-0.035$, $+0.012$] \\
2 draws \at{4}{3} ($3{,}840$) $-$ 1 draw \at{4}{50} ($47{,}040$) & $-0.127$\sig [$-0.162$, $-0.095$] & $-0.187$\sig [$-0.243$, $-0.128$] & $-0.034$\sig [$-0.061$, $-0.010$] \\
\midrule
\multicolumn{4}{@{}l}{\emph{Four-draw score averaging at two steps ($S{=}2$, $3{,}840$ evaluations, seeds 0--2)}} \\
4 draws \at{1}{2} ($3{,}840$) $-$ 1 draw \at{1}{5} ($3{,}840$) & $-0.010$ [$-0.038$, $+0.020$] & $+0.008$ [$-0.062$, $+0.084$] & $-0.012$ [$-0.040$, $+0.013$] \\
4 draws \at{1}{2} ($3{,}840$) $-$ 2 draws \at{1}{3} ($3{,}840$) & $+0.016$ [$-0.004$, $+0.038$] & $+0.130$\sig [$+0.066$, $+0.192$] & $-0.005$ [$-0.028$, $+0.017$] \\
4 draws \at{1}{2} ($3{,}840$) $-$ 1 draw \at{1}{2} (mean over 4 draws) & $+0.006$ [$-0.002$, $+0.014$] & $-0.036$\sig [$-0.056$, $-0.015$] & $-0.002$ [$-0.010$, $+0.007$] \\
4 draws \monoat{2} ($3{,}840$) $-$ 1 draw \monoat{5} ($3{,}840$) & $-0.033$\sig [$-0.064$, $-0.003$] & $-0.094$\sig [$-0.158$, $-0.024$] & $+0.056$\sig [$+0.026$, $+0.085$] \\
4 draws \monoat{2} ($3{,}840$) $-$ 2 draws \monoat{3} ($3{,}840$) & $+0.008$ [$-0.017$, $+0.033$] & $+0.072$\sig [$+0.012$, $+0.130$] & $+0.036$\sig [$+0.013$, $+0.059$] \\
4 draws \monoat{2} ($3{,}840$) $-$ 1 draw \monoat{2} (mean over 4 draws) & $-0.001$ [$-0.009$, $+0.007$] & $-0.029$\sig [$-0.048$, $-0.009$] & $-0.003$ [$-0.011$, $+0.005$] \\
\midrule
\multicolumn{4}{@{}l}{\emph{Three-seed multi-draw score averaging at five steps (\at{1}{5}, $M{=}3$, seeds 0--2) and seed-0 \at{1}{50} ($n{=}500$)}} \\
2 draws \at{1}{3} ($3{,}840$) $-$ 2 draws \at{1}{5} ($7{,}680$) & $-0.011$ [$-0.029$, $+0.007$] & $-0.012$ [$-0.049$, $+0.029$] & $+0.003$ [$-0.017$, $+0.020$] \\
2 draws \at{1}{3} ($3{,}840$) $-$ 3 draws \at{1}{5} ($11{,}520$) & $-0.007$ [$-0.029$, $+0.014$] & $+0.035$ [$-0.011$, $+0.079$] & $+0.005$ [$-0.017$, $+0.028$] \\
2 draws \at{1}{5} ($7{,}680$) $-$ 1 draw \at{1}{5} (mean over 3 draws) & $-0.026$\sig [$-0.035$, $-0.017$] & $-0.116$\sig [$-0.139$, $-0.092$] & $-0.003$ [$-0.014$, $+0.008$] \\
3 draws \at{1}{5} ($11{,}520$) $-$ 1 draw \at{1}{5} (mean over 3 draws) & $-0.030$\sig [$-0.045$, $-0.017$] & $-0.162$\sig [$-0.196$, $-0.126$] & $-0.006$ [$-0.021$, $+0.010$] \\
3 draws \at{1}{5} ($11{,}520$) $-$ 1 draw \at{1}{50} ($47{,}040$) & $-0.120$\sig [$-0.147$, $-0.093$] & $-0.244$\sig [$-0.298$, $-0.185$] & $-0.027$\sig [$-0.053$, $-0.004$] \\
Seed 0: 3 draws \at{1}{50} ($141{,}120$) $-$ 1 draw \at{1}{50} (mean over 3 draws) & $-0.038$\sig [$-0.070$, $-0.006$] & $-0.183$\sig [$-0.245$, $-0.113$] & -- \\
Seed 0: 3 draws \at{1}{50} ($141{,}120$) $-$ 2 draws \at{1}{3} ($3{,}840$) & $+0.105$\sig [$+0.058$, $+0.151$] & $+0.024$ [$-0.071$, $+0.114$] & -- \\
Seed 0: 3 draws \at{1}{50} ($141{,}120$) $-$ 1 draw \at{1}{5} (mean over 3 draws) & $+0.071$\sig [$+0.034$, $+0.109$] & $-0.092$\sig [$-0.165$, $-0.022$] & -- \\
Seed 0: 3 draws \at{1}{50} ($141{,}120$) $-$ 3 draws \at{1}{5} ($11{,}520$) & $+0.094$\sig [$+0.051$, $+0.134$] & $+0.035$ [$-0.044$, $+0.111$] & -- \\
\midrule
\multicolumn{4}{@{}l}{\emph{Three-draw second-order solvers vs.\ three-draw five-step Euler (seed 0, $n{=}100$ nested shard 0/5)}} \\
Seed 0 ($n{=}100$): 3 draws \M{1} Heun@3 $-$ 3 draws \at{1}{5} ($11{,}520$) & $+0.157$\sig [$+0.064$, $+0.248$] & $+0.258$\sig [$+0.097$, $+0.430$] & $-0.034$ [$-0.117$, $+0.046$] \\
Seed 0 ($n{=}100$): 3 draws \M{1} midpoint@3 $-$ 3 draws \at{1}{5} ($11{,}520$) & $+0.112$\sig [$+0.030$, $+0.193$] & $+0.056$ [$-0.080$, $+0.199$] & $-0.008$ [$-0.087$, $+0.071$] \\
