# Supplementary material for: Fewer Steps, Better Plans: Sampling Variance in Flow-Matching Navigation World Models
Source: arXiv:2611.36153 source file (2026-11-26)
Supplement: Supplementary file 18 [file supp_sdpa_shard_body.tex]

\mono & 50 / 49 & 80.9 (1.0$\times$) & -- & -- & 52.1 (1.0$\times$) & 51.9$^{\dagger}$ (1.0$\times$) & 187.4 (1.0$\times$) & 2.805 / 2.789 & $+0.559^{\dagger}$ \ci{$-0.016$, $+1.102$} \\
\paper \M{4} & 50 / 49 & 80.8 (1.0$\times$) & -- & -- & 53.2 (1.0$\times$) & 53.2$^{\dagger}$ (1.0$\times$) & 187.7 (1.0$\times$) & 2.679 / 2.698 & $+0.320^{\dagger}$ \ci{$-0.122$, $+0.799$} \\
\paper \M{1} & 50 / 49 & 68.8 (1.2$\times$) & -- & -- & 39.8 (1.3$\times$) & 39.8$^{\dagger}$ (1.3$\times$) & 176.1 (1.1$\times$) & 2.947 / 2.941 & $+0.176^{\dagger}$ \ci{$-0.283$, $+0.599$} \\
\midrule
\mono & 5 / 4 & 6.92 (11.7$\times$) & 6.70 & 4.64 & 4.40 (11.8$\times$) & 4.30 (12.1$\times$) & 15.7 (11.9$\times$) & 2.873 / 2.886 & $-0.158$ \ci{$-0.430$, $+0.104$} \\
\paper \M{4} & 5 / 4 & 6.97 (11.6$\times$) & 6.73 & 4.69 & 4.44 (11.7$\times$) & 4.37 (11.9$\times$) & 15.7 (11.9$\times$) & 2.948 / 2.948 & $-0.176$ \ci{$-0.415$, $+0.080$} \\
\paper \M{1} & 5 / 4 & 5.91 (13.7$\times$) & 5.65 & 3.60 & 3.35 (15.6$\times$) & 3.27 (15.9$\times$) & 14.8 (12.7$\times$) & 2.724 / 2.741 & $-0.069$ \ci{$-0.335$, $+0.172$} \\
\midrule
\mono (2 draws) & 3 / 2 & 7.23 (11.2$\times$) & 6.74 & 4.95 & 4.48 (11.6$\times$) & 4.26 (12.2$\times$) & 16.0 (11.7$\times$) & 2.776 / 2.736 & $-0.017$ \ci{$-0.215$, $+0.188$} \\
\paper \M{4} (2 draws) & 3 / 2 & 7.27 (11.1$\times$) & 6.77 & 5.02 & 4.49 (11.6$\times$) & 4.35 (11.9$\times$) & 16.1 (11.6$\times$) & 2.789 / 2.789 & $+0.143$ \ci{$-0.068$, $+0.359$} \\
\paper \M{1} (2 draws) & 3 / 2 & 6.17 (13.1$\times$) & 5.66 & 3.90 & 3.39 (15.4$\times$) & 3.24 (16.0$\times$) & 15.1 (12.4$\times$) & 2.686 / 2.686 & $+0.155$ \ci{$-0.040$, $+0.342$} \\
\midrule
\mono & 3 / 2 & 3.64 (22.2$\times$) & 3.42 & 2.48 & 2.26 (23.0$\times$) & 2.15 (24.1$\times$) & 8.01 (23.4$\times$) & 2.931 / 2.917 & $-0.156$ \ci{$-0.364$, $+0.042$} \\
\paper \M{4} & 3 / 2 & 3.66 (22.1$\times$) & 3.42 & 2.51 & 2.26 (23.1$\times$) & 2.19 (23.7$\times$) & 8.08 (23.2$\times$) & 2.940 / 2.986 & $+0.022$ \ci{$-0.246$, $+0.264$} \\
\paper \M{1} & 3 / 2 & 3.13 (25.8$\times$) & 2.88 & 1.98 & 1.72 (30.3$\times$) & 1.64 (31.6$\times$) & 7.57 (24.8$\times$) & 2.789 / 2.789 & $+0.051$ \ci{$-0.162$, $+0.276$} \\
\midrule
\mono & 2 / 1 & 1.98 (40.8$\times$) & 1.78 & 1.59 & 1.19 (43.8$\times$) & 1.08 (47.9$\times$) & 4.19 (44.7$\times$) & 2.894 / 2.919 & $-0.202$ \ci{$-0.409$, $+0.001$} \\
\paper \M{4} & 2 / 1 & 2.00 (40.4$\times$) & 1.76 & 1.60 & 1.17 (44.4$\times$) & 1.10 (47.1$\times$) & 4.22 (44.4$\times$) & 2.785 / 2.797 & $+0.091$ \ci{$-0.106$, $+0.293$} \\
\paper \M{1} & 2 / 1 & 1.78 (45.4$\times$) & 1.49 & 1.60 & 0.91 (57.4$\times$) & 0.83 (62.6$\times$) & 3.96 (47.3$\times$) & 2.660 / 2.663 & $+0.062$ \ci{$-0.173$, $+0.260$} \\
