# Supplementary material for: Fewer Steps, Better Plans: Sampling Variance in Flow-Matching Navigation World Models
Source: arXiv:2611.36153 source file (2026-11-26)
Supplement: Supplementary file 19 [file supp_seeds_body.tex]

All-\M{1} & 50 & 1.37 / 1.39 / 1.34 ($1.37\pm0.02$) & 2.78 / 2.89 / 2.84 ($2.84\pm0.06$) & 1.01 / 1.02 / 1.04 ($1.03\pm0.01$) \\
 & 20 & 1.34 / 1.36 / 1.33 ($1.35\pm0.02$) & 2.79 / 2.87 / 2.84 ($2.83\pm0.04$) & 1.02 / 1.03 / 1.07 ($1.04\pm0.03$) \\
 & 10 & 1.32 / 1.32 / 1.30 ($1.31\pm0.01$) & 2.74 / 2.83 / 2.76 ($2.78\pm0.05$) & 0.99 / 1.01 / 1.05 ($1.02\pm0.03$) \\
 & 5 & 1.26 / 1.26 / 1.28 ($1.27\pm0.02$) & 2.68 / 2.83 / 2.74 ($2.75\pm0.08$) & 1.00 / 1.00 / 1.03 ($1.01\pm0.01$) \\
 & 5, 2 draws & 1.25 / 1.26 / 1.24 ($1.25\pm0.01$) & 2.63 / 2.68 / 2.60 ($2.64\pm0.04$) & 1.01 / 0.97 / 1.03 ($1.00\pm0.03$) \\
 & 5, 3 draws & 1.25 / 1.26 / 1.24 ($1.25\pm0.01$) & 2.60 / 2.62 / 2.56 ($2.59\pm0.03$) & 1.01 / 0.97 / 1.02 ($1.00\pm0.03$) \\
 & 4 & 1.27 / 1.26 / 1.25 ($1.26\pm0.01$) & 2.67 / 2.79 / 2.68 ($2.71\pm0.07$) & 1.00 / 1.00 / 1.02 ($1.01\pm0.01$) \\
 & 3 & 1.24 / 1.25 / 1.25 ($1.25\pm0.00$) & 2.67 / 2.74 / 2.73 ($2.71\pm0.04$) & 1.01 / 0.97 / 1.01 ($1.00\pm0.02$) \\
 & 3, 2 draws & 1.24 / 1.24 / 1.25 ($1.24\pm0.01$) & 2.61 / 2.66 / 2.61 ($2.63\pm0.03$) & 1.01 / 0.97 / 1.03 ($1.00\pm0.03$) \\
 & 3, Heun & 1.41 / 1.41 / 1.41 ($1.41\pm0.00$) & 2.80 / 2.83 / 2.77 ($2.80\pm0.03$) & 0.99 / 1.00 / 1.03 ($1.01\pm0.02$) \\
 & 3, midpoint & 1.37 / 1.38 / 1.36 ($1.37\pm0.01$) & 2.78 / 2.85 / 2.75 ($2.79\pm0.05$) & 1.01 / 1.03 / 1.05 ($1.03\pm0.02$) \\
 & unif.\ Euler ($\alpha{=}1$) & 1.27 / 1.29 / 1.29 ($1.28\pm0.01$) & 2.70 / 2.78 / 2.72 ($2.73\pm0.04$) & 0.99 / 0.99 / 1.02 ($1.00\pm0.02$) \\
 & unif.\ Heun ($\alpha{=}1$) & 1.33 / 1.34 / 1.33 ($1.34\pm0.01$) & 2.75 / 2.78 / 2.74 ($2.75\pm0.02$) & 1.01 / 1.01 / 1.05 ($1.02\pm0.02$) \\
 & unif.\ midpoint ($\alpha{=}1$) & 1.36 / 1.40 / 1.36 ($1.37\pm0.02$) & 2.75 / 2.79 / 2.70 ($2.74\pm0.05$) & 1.01 / 1.00 / 1.07 ($1.03\pm0.03$) \\
 & 2 & 1.26 / 1.24 / 1.25 ($1.25\pm0.01$) & 2.80 / 2.79 / 2.84 ($2.81\pm0.03$) & 0.99 / 0.99 / 1.01 ($1.00\pm0.01$) \\
 & 2, 4 draws & 1.26 / 1.26 / 1.25 ($1.26\pm0.01$) & 2.77 / 2.74 / 2.77 ($2.76\pm0.02$) & 1.00 / 0.97 / 1.02 ($1.00\pm0.02$) \\
\midrule
All-\M{4} & 50 & 1.38 / 1.37 / 1.34 ($1.36\pm0.02$) & 2.81 / 2.88 / 2.81 ($2.83\pm0.04$) & 1.02 / 1.00 / 1.06 ($1.03\pm0.03$) \\
 & 5 & 1.27 / 1.29 / 1.25 ($1.27\pm0.02$) & 2.71 / 2.79 / 2.81 ($2.77\pm0.05$) & 1.00 / 0.99 / 1.02 ($1.01\pm0.02$) \\
 & 3 & 1.25 / 1.25 / 1.25 ($1.25\pm0.00$) & 2.69 / 2.76 / 2.77 ($2.74\pm0.04$) & 1.01 / 0.99 / 1.03 ($1.01\pm0.02$) \\
 & 3, 2 draws & 1.25 / 1.24 / 1.22 ($1.24\pm0.02$) & 2.68 / 2.62 / 2.63 ($2.64\pm0.03$) & 1.01 / 0.96 / 1.01 ($0.99\pm0.03$) \\
 & 2 & 1.25 / 1.25 / 1.23 ($1.24\pm0.01$) & 2.76 / 2.75 / 2.76 ($2.76\pm0.01$) & 0.99 / 0.99 / 1.01 ($1.00\pm0.01$) \\
\midrule
\mono & 50 & 1.35 / 1.37 / 1.37 ($1.36\pm0.01$) & 2.85 / 2.81 / 2.86 ($2.84\pm0.02$) & 1.01 / 1.05 / 1.05 ($1.04\pm0.02$) \\
 & 20 & 1.35 / 1.34 / 1.36 ($1.35\pm0.01$) & 2.85 / 2.78 / 2.82 ($2.82\pm0.04$) & 1.03 / 1.05 / 1.07 ($1.05\pm0.02$) \\
 & 10 & 1.32 / 1.35 / 1.31 ($1.33\pm0.02$) & 2.80 / 2.72 / 2.80 ($2.77\pm0.05$) & 1.00 / 1.04 / 1.05 ($1.03\pm0.03$) \\
 & 5 & 1.29 / 1.31 / 1.28 ($1.30\pm0.01$) & 2.78 / 2.72 / 2.78 ($2.76\pm0.03$) & 1.01 / 1.03 / 1.05 ($1.03\pm0.02$) \\
 & 4 & 1.29 / 1.29 / 1.28 ($1.28\pm0.01$) & 2.72 / 2.66 / 2.72 ($2.70\pm0.04$) & 1.04 / 1.01 / 1.05 ($1.03\pm0.02$) \\
 & 3 & 1.27 / 1.29 / 1.25 ($1.27\pm0.02$) & 2.73 / 2.62 / 2.64 ($2.66\pm0.06$) & 1.07 / 1.05 / 1.05 ($1.06\pm0.01$) \\
 & 3, 2 draws & 1.26 / 1.27 / 1.23 ($1.25\pm0.02$) & 2.61 / 2.55 / 2.61 ($2.59\pm0.03$) & 1.06 / 1.04 / 1.05 ($1.05\pm0.01$) \\
 & 3, Heun & 1.38 / 1.39 / 1.39 ($1.39\pm0.00$) & 2.83 / 2.80 / 2.82 ($2.81\pm0.01$) & 1.05 / 1.06 / 1.06 ($1.06\pm0.01$) \\
 & 3, midpoint & 1.39 / 1.38 / 1.36 ($1.38\pm0.01$) & 2.78 / 2.70 / 2.77 ($2.75\pm0.04$) & 1.03 / 1.03 / 1.06 ($1.04\pm0.02$) \\
 & unif.\ Euler ($\alpha{=}1$) & 1.30 / 1.32 / 1.31 ($1.31\pm0.01$) & 2.75 / 2.64 / 2.67 ($2.69\pm0.06$) & 1.01 / 1.04 / 1.07 ($1.04\pm0.03$) \\
 & unif.\ Heun ($\alpha{=}1$) & 1.34 / 1.36 / 1.36 ($1.35\pm0.01$) & 2.73 / 2.70 / 2.71 ($2.71\pm0.02$) & 1.01 / 1.05 / 1.06 ($1.04\pm0.03$) \\
 & unif.\ midpoint ($\alpha{=}1$) & 1.37 / 1.40 / 1.39 ($1.39\pm0.02$) & 2.79 / 2.68 / 2.71 ($2.73\pm0.06$) & 1.04 / 1.03 / 1.07 ($1.05\pm0.02$) \\
 & 2 & 1.26 / 1.27 / 1.26 ($1.26\pm0.00$) & 2.71 / 2.67 / 2.75 ($2.71\pm0.04$) & 1.10 / 1.08 / 1.11 ($1.09\pm0.02$) \\
 & 2, 4 draws & 1.26 / 1.26 / 1.26 ($1.26\pm0.00$) & 2.66 / 2.64 / 2.69 ($2.66\pm0.02$) & 1.08 / 1.09 / 1.09 ($1.09\pm0.00$) \\
\midrule
Standalone \M{1} & 50 & 1.36 / 1.38 / 1.37 ($1.37\pm0.01$) & 2.83 / 2.82 / 2.83 ($2.83\pm0.00$) & 1.00 / 1.01 / 1.05 ($1.02\pm0.02$) \\
 & 5 & 1.28 / 1.29 / 1.27 ($1.28\pm0.01$) & 2.69 / 2.73 / 2.73 ($2.72\pm0.02$) & 0.98 / 0.99 / 1.00 ($0.99\pm0.01$) \\
\midrule
Standalone \M{0} & 50 & 1.42 / 1.41 / 1.38 ($1.40\pm0.02$) & 3.01 / 3.00 / 3.05 ($3.02\pm0.02$) & 1.01 / 1.01 / 1.05 ($1.02\pm0.02$) \\
 & 5 & 1.27 / 1.26 / 1.26 ($1.26\pm0.01$) & 2.87 / 2.91 / 2.97 ($2.92\pm0.05$) & 0.99 / 1.01 / 1.02 ($1.01\pm0.02$) \\
 & 3 & 1.27 / 1.26 / 1.31 ($1.28\pm0.03$) & 2.87 / 2.92 / 2.94 ($2.91\pm0.03$) & 0.99 / 1.02 / 1.00 ($1.01\pm0.01$) \\
 & 2 & 1.27 / 1.29 / 1.29 ($1.29\pm0.01$) & 2.91 / 2.93 / 2.92 ($2.92\pm0.01$) & 1.02 / 1.03 / 1.00 ($1.01\pm0.02$) \\
\midrule
\mono, naive \M{1} slice & 5 & 1.73 / -- / -- (1.73) & 4.86 / -- / -- (4.86) & 1.09 / -- / -- (1.09) \\
