# Supplementary material for: Fewer Steps, Better Plans: Sampling Variance in Flow-Matching Navigation World Models
Source: arXiv:2611.36153 source file (2026-11-26)
Supplement: Supplementary file 20 [file supp_t13_body.tex]

\multicolumn{7}{@{}l}{\emph{(a) Two-round iterative \cem (2\,s / 8-step horizon; round 0 = 1-round plan inside the same job)}} \\
\paper \M{1} & \recon & 1.350 / 1.318 & 1.268 / 1.226 & $-0.101$\sig [$-0.153$, $-0.047$] & $-0.107$\sig [$-0.188$, $-0.037$] & $-0.042$\sig [$-0.062$, $-0.021$] / $-0.033$ [$-0.093$, $+0.028$] \\
\paper \M{1} & \sacson & 2.792 / 2.693 & 2.754 / 2.584 & $-0.096$ [$-0.213$, $+0.023$] & $-0.171$\sig [$-0.309$, $-0.030$] & $-0.170$\sig [$-0.239$, $-0.106$] / $-0.099$ [$-0.261$, $+0.053$] \\
\mono & \recon & 1.416 / 1.394 & 1.290 / 1.265 & $-0.110$\sig [$-0.162$, $-0.063$] & $-0.125$\sig [$-0.199$, $-0.059$] & $-0.024$\sig [$-0.045$, $-0.004$] / $-0.022$ [$-0.077$, $+0.031$] \\
\mono & \sacson & 2.738 / 2.580 & 2.753 / 2.599 & $-0.048$ [$-0.147$, $+0.060$] & $+0.017$ [$-0.104$, $+0.140$] & $-0.153$\sig [$-0.219$, $-0.091$] / $-0.158$ [$-0.325$, $+0.002$] \\
\midrule
\multicolumn{7}{@{}l}{\emph{(b) Longer planning horizon: 4\,s / 16 autoregressive steps (1-round \cem; \ate / \rpe and paired $S{=}5 - S{=}50$ on $n{=}100$)}} \\
\paper \M{1} & \recon & 3.347 / 0.537 & 3.234 / 0.524 & $+0.020$ [$-0.101$, $+0.143$] & $+0.015$\sig [$+0.004$, $+0.027$] & -- \\
\paper \M{1} & \sacson & 5.413 / 0.748 & 5.339 / 0.749 & $+0.042$ [$-0.152$, $+0.237$] & $+0.003$ [$-0.018$, $+0.024$] & -- \\
\mono & \recon & 3.366 / 0.538 & 3.210 / 0.519 & $+0.009$ [$-0.120$, $+0.137$] & $+0.011$\sig [$+0.001$, $+0.021$] & -- \\
\mono & \sacson & 5.441 / 0.748 & 5.343 / 0.744 & $+0.040$ [$-0.144$, $+0.231$] & $+0.003$ [$-0.013$, $+0.019$] & -- \\
