# Supplementary material for: Fewer Steps, Better Plans: Sampling Variance in Flow-Matching Navigation World Models
Source: arXiv:2611.36153 source file (2026-11-26)
Supplement: Supplementary file 21 [file supp_t2_reg_gen_body.tex]

\recon & DINO-Reg, 25 epochs & 0.4997 & 0.5815 & 0.4809 & 0.5584 & 167.54 & 217.73 \\
 & DINO-Reg, 47 epochs & 0.4669 & 0.5565 & 0.4482 & 0.5218 & 118.72 & 154.48 \\
 & DINO-Reg, 50 epochs & 0.4644 & 0.5542 & 0.4462 & 0.5195 & 115.51 & 149.71 \\
 & \paper \M{1}, $S{=}50$ & 0.3846 & 0.4602 & 0.4221 & 0.4783 & 20.29 & 20.26 \\
\midrule
\sacson & DINO-Reg, 25 epochs & 0.4173 & 0.4568 & 0.4195 & 0.4679 & 124.55 & 149.24 \\
 & DINO-Reg, 47 epochs & 0.3886 & 0.4294 & 0.3842 & 0.4288 & 100.55 & 122.86 \\
 & DINO-Reg, 50 epochs & 0.3865 & 0.4275 & 0.3817 & 0.4266 & 98.76 & 120.85 \\
 & \paper \M{1}, $S{=}50$ & 0.3433 & 0.3786 & 0.3618 & 0.3916 & 19.12 & 20.96 \\
\midrule
\scand & DINO-Reg, 25 epochs & 0.5289 & 0.5640 & 0.4846 & 0.5196 & 134.97 & 144.72 \\
 & DINO-Reg, 47 epochs & 0.4884 & 0.5191 & 0.4783 & 0.5100 & 98.44 & 103.41 \\
 & DINO-Reg, 50 epochs & 0.4847 & 0.5146 & 0.4785 & 0.5100 & 95.23 & 99.81 \\
 & \paper \M{1}, $S{=}50$ & 0.3991 & 0.4587 & 0.4564 & 0.5151 & 31.12 & 35.65 \\
\midrule
Mean & DINO-Reg, 25 epochs & 0.4820 & 0.5341 & 0.4617 & 0.5153 & 142.35 & 170.57 \\
 & DINO-Reg, 47 epochs & 0.4480 & 0.5017 & 0.4369 & 0.4869 & 105.90 & 126.92 \\
 & DINO-Reg, 50 epochs & 0.4452 & 0.4988 & 0.4355 & 0.4854 & 103.16 & 123.46 \\
 & \paper \M{1}, $S{=}50$ & 0.3757 & 0.4325 & 0.4134 & 0.4617 & 23.51 & 25.62 \\
