# Supplementary material for: Fewer Steps, Better Plans: Sampling Variance in Flow-Matching Navigation World Models
Source: arXiv:2611.36153 source file (2026-11-26)
Supplement: Supplementary file 22 [file supp_t2_reg_plan_body.tex]

DINO-Reg, 25 epochs & $1.753\pm0.018$ & $2.965\pm0.058$ & $1.229\pm0.026$ & $0.449\pm0.005$ & $0.731\pm0.007$ & $0.318\pm0.005$ \\
DINO-Reg, 47 epochs & $2.198\pm0.026$ & $3.080\pm0.022$ & $1.230\pm0.026$ & $0.538\pm0.005$ & $0.750\pm0.003$ & $0.318\pm0.006$ \\
DINO-Reg, 50 epochs (Table~2) & $2.234\pm0.005$ & $3.090\pm0.033$ & $1.223\pm0.024$ & $0.544\pm0.002$ & $0.755\pm0.004$ & $0.318\pm0.005$ \\
\addlinespace[2pt]
\paper \M{1}, $S{=}2$ (1 NFE) & $1.249\pm0.010$ & $2.811\pm0.027$ & $0.996\pm0.012$ & $0.376\pm0.003$ & $0.705\pm0.005$ & $0.284\pm0.002$ \\
\paper \M{1}, $S{=}5$ (4 NFEs) & $1.266\pm0.016$ & $2.749\pm0.077$ & $1.011\pm0.014$ & $0.363\pm0.001$ & $0.692\pm0.015$ & $0.283\pm0.001$ \\
\mono, $S{=}50$ (49 NFEs) & $1.363\pm0.010$ & $2.838\pm0.024$ & $1.038\pm0.023$ & $0.367\pm0.001$ & $0.698\pm0.003$ & $0.288\pm0.002$ \\
