# Supplementary material for: Fewer Steps, Better Plans: Sampling Variance in Flow-Matching Navigation World Models
Source: arXiv:2611.36153 source file (2026-11-26)
Supplement: Supplementary file 23 [file supp_t2_reg_plan_ci_body.tex]

\multicolumn{4}{@{}l}{\emph{\ate}} \\
DINO-Reg (50) $-$ \M{1}@2 (1 NFE) & $+0.985$\sig [$+0.895$, $+1.072$] & $+0.280$\sig [$+0.186$, $+0.374$] & $+0.227$\sig [$+0.192$, $+0.265$] \\
DINO-Reg (50) $-$ \M{1}@5 (4 NFEs) & $+0.967$\sig [$+0.887$, $+1.050$] & $+0.342$\sig [$+0.259$, $+0.432$] & $+0.213$\sig [$+0.178$, $+0.248$] \\
DINO-Reg (50) $-$ {\mono}@50 (49 NFEs) & $+0.871$\sig [$+0.796$, $+0.948$] & $+0.253$\sig [$+0.165$, $+0.342$] & $+0.185$\sig [$+0.148$, $+0.219$] \\
DINO-Reg (50) $-$ DINO-Reg (47) & $+0.036$\sig [$+0.018$, $+0.054$] & $+0.011$ [$-0.019$, $+0.041$] & $-0.007$ [$-0.018$, $+0.006$] \\
DINO-Reg (50) $-$ DINO-Reg (25) & $+0.480$\sig [$+0.414$, $+0.545$] & $+0.126$\sig [$+0.060$, $+0.192$] & $-0.006$ [$-0.038$, $+0.026$] \\
DINO-Reg (47) $-$ DINO-Reg (25) & $+0.445$\sig [$+0.379$, $+0.506$] & $+0.115$\sig [$+0.053$, $+0.180$] & $+0.000$ [$-0.031$, $+0.031$] \\
\midrule
\multicolumn{4}{@{}l}{\emph{\rpe}} \\
DINO-Reg (50) $-$ \M{1}@2 (1 NFE) & $+0.168$\sig [$+0.154$, $+0.183$] & $+0.050$\sig [$+0.034$, $+0.064$] & $+0.034$\sig [$+0.028$, $+0.041$] \\
DINO-Reg (50) $-$ \M{1}@5 (4 NFEs) & $+0.181$\sig [$+0.166$, $+0.196$] & $+0.063$\sig [$+0.048$, $+0.079$] & $+0.035$\sig [$+0.029$, $+0.040$] \\
DINO-Reg (50) $-$ {\mono}@50 (49 NFEs) & $+0.177$\sig [$+0.164$, $+0.192$] & $+0.057$\sig [$+0.041$, $+0.073$] & $+0.030$\sig [$+0.025$, $+0.036$] \\
DINO-Reg (50) $-$ DINO-Reg (47) & $+0.006$\sig [$+0.003$, $+0.010$] & $+0.005$ [$-0.001$, $+0.011$] & $-0.000$ [$-0.002$, $+0.002$] \\
DINO-Reg (50) $-$ DINO-Reg (25) & $+0.095$\sig [$+0.084$, $+0.107$] & $+0.024$\sig [$+0.011$, $+0.037$] & $-0.000$ [$-0.005$, $+0.005$] \\
DINO-Reg (47) $-$ DINO-Reg (25) & $+0.089$\sig [$+0.078$, $+0.100$] & $+0.019$\sig [$+0.007$, $+0.032$] & $+0.000$ [$-0.005$, $+0.005$] \\
