# Supplementary material for: Fewer Steps, Better Plans: Sampling Variance in Flow-Matching Navigation World Models
Source: arXiv:2611.36153 source file (2026-11-26)
Supplement: Supplementary file 24 [file supp_t2_reg_tok_body.tex]

\multicolumn{16}{@{}l}{\emph{1\,s: one-shot prediction vs.\ frame 3 of the rollout (four chained 0.25\,s steps, 1.00\,s)}} \\
DINO-Reg, 25 epochs & 0.167 & 0.184 & $+0.017$ & 0.380 & 0.416 & 0.137 & 0.150 & $+0.013$ & 0.321 & 0.350 & 0.241 & 0.271 & $+0.030$ & 0.542 & 0.610 \\
DINO-Reg, 47 epochs & 0.167 & 0.184 & $+0.017$ & 0.380 & 0.417 & 0.133 & 0.148 & $+0.015$ & 0.313 & 0.346 & 0.266 & 0.292 & $+0.026$ & 0.603 & 0.665 \\
DINO-Reg, 50 epochs & 0.167 & 0.184 & $+0.016$ & 0.381 & 0.417 & 0.133 & 0.148 & $+0.015$ & 0.313 & 0.346 & 0.269 & 0.294 & $+0.026$ & 0.610 & 0.671 \\
\addlinespace[2pt]
\M{1}, $S{=}2$ (1) & 0.170 & 0.181 & $+0.011$ & 0.385 & 0.408 & 0.145 & 0.156 & $+0.011$ & 0.338 & 0.361 & 0.191 & 0.206 & $+0.015$ & 0.436 & 0.471 \\
\M{1}, $S{=}3$ (2) & 0.198 & 0.207 & $+0.009$ & 0.453 & 0.474 & 0.164 & 0.174 & $+0.010$ & 0.386 & 0.408 & 0.216 & 0.227 & $+0.011$ & 0.499 & 0.526 \\
\M{1}, $S{=}5$ (4) & 0.228 & 0.235 & $+0.008$ & 0.534 & 0.554 & 0.188 & 0.196 & $+0.008$ & 0.449 & 0.469 & 0.243 & 0.249 & $+0.006$ & 0.575 & 0.592 \\
\M{1}, $S{=}50$ (49) & 0.272 & 0.282 & $+0.010$ & 0.667 & 0.692 & 0.229 & 0.237 & $+0.008$ & 0.569 & 0.589 & 0.286 & 0.287 & $+0.001$ & 0.711 & 0.715 \\
\midrule
\multicolumn{16}{@{}l}{\emph{2\,s: one-shot prediction vs.\ frame 8 of the rollout (nine chained 0.25\,s steps, 2.25\,s)}} \\
DINO-Reg, 25 epochs & 0.174 & 0.226 & $+0.052$ & 0.394 & 0.504 & 0.137 & 0.174 & $+0.037$ & 0.320 & 0.401 & 0.249 & 0.305 & $+0.056$ & 0.559 & 0.685 \\
DINO-Reg, 47 epochs & 0.175 & 0.228 & $+0.053$ & 0.397 & 0.513 & 0.133 & 0.178 & $+0.045$ & 0.312 & 0.413 & 0.271 & 0.322 & $+0.051$ & 0.614 & 0.736 \\
DINO-Reg, 50 epochs & 0.175 & 0.228 & $+0.053$ & 0.398 & 0.514 & 0.133 & 0.178 & $+0.045$ & 0.313 & 0.414 & 0.274 & 0.324 & $+0.050$ & 0.621 & 0.741 \\
\addlinespace[2pt]
\M{1}, $S{=}2$ (1) & 0.178 & 0.212 & $+0.035$ & 0.402 & 0.476 & 0.146 & 0.176 & $+0.030$ & 0.342 & 0.406 & 0.208 & 0.249 & $+0.040$ & 0.472 & 0.564 \\
\M{1}, $S{=}3$ (2) & 0.207 & 0.239 & $+0.032$ & 0.474 & 0.548 & 0.166 & 0.191 & $+0.026$ & 0.390 & 0.449 & 0.236 & 0.270 & $+0.034$ & 0.541 & 0.623 \\
\M{1}, $S{=}5$ (4) & 0.238 & 0.267 & $+0.029$ & 0.558 & 0.629 & 0.190 & 0.213 & $+0.023$ & 0.454 & 0.509 & 0.265 & 0.291 & $+0.026$ & 0.624 & 0.691 \\
\M{1}, $S{=}50$ (49) & 0.282 & 0.314 & $+0.031$ & 0.691 & 0.770 & 0.233 & 0.252 & $+0.019$ & 0.577 & 0.626 & 0.310 & 0.328 & $+0.019$ & 0.768 & 0.819 \\
