# Supplementary material for: Fewer Steps, Better Plans: Sampling Variance in Flow-Matching Navigation World Models
Source: arXiv:2611.36153 source file (2026-11-26)
Supplement: Supplementary file 25 [file supp_t2_reg_turns_body.tex]

\recon & Q1 straightest (0.07--1.14) & 0.89 & 1.087 & 1.075 & 1.048 & 1.053 & 1.232 & 1.205 & 1.210 & $+0.134$\sig \ci{$+0.061$, $+0.203$} & $+0.162$\sig \ci{$+0.077$, $+0.248$} & $+0.157$\sig \ci{$+0.082$, $+0.236$} \\
 & Q2 (1.15--2.20) & 1.25 & 1.161 & 1.132 & 1.139 & 1.116 & 1.419 & 1.629 & 1.671 & $+0.539$\sig \ci{$+0.427$, $+0.654$} & $+0.532$\sig \ci{$+0.419$, $+0.648$} & $+0.555$\sig \ci{$+0.445$, $+0.672$} \\
 & Q3 (2.20--3.53) & 1.73 & 1.314 & 1.155 & 1.172 & 1.140 & 1.577 & 2.321 & 2.369 & $+1.214$\sig \ci{$+1.084$, $+1.330$} & $+1.197$\sig \ci{$+1.062$, $+1.321$} & $+1.229$\sig \ci{$+1.102$, $+1.355$} \\
 & Q4 sharpest (3.54--8.95) & 2.68 & 1.889 & 1.703 & 1.639 & 1.653 & 2.786 & 3.638 & 3.686 & $+1.983$\sig \ci{$+1.835$, $+2.118$} & $+2.048$\sig \ci{$+1.882$, $+2.195$} & $+2.033$\sig \ci{$+1.861$, $+2.190$} \\
\midrule
\sacson & Q1 straightest (0.00--0.60) & 2.67 & 1.747 & 1.644 & 1.688 & 1.469 & 1.875 & 1.953 & 1.959 & $+0.315$\sig \ci{$+0.169$, $+0.458$} & $+0.271$\sig \ci{$+0.125$, $+0.416$} & $+0.490$\sig \ci{$+0.344$, $+0.633$} \\
 & Q2 (0.61--1.49) & 3.60 & 2.693 & 2.690 & 2.701 & 2.538 & 2.881 & 2.878 & 2.921 & $+0.232$\sig \ci{$+0.054$, $+0.392$} & $+0.220$\sig \ci{$+0.068$, $+0.382$} & $+0.383$\sig \ci{$+0.218$, $+0.557$} \\
 & Q3 (1.51--3.28) & 3.92 & 3.028 & 2.890 & 2.924 & 2.758 & 3.092 & 3.371 & 3.346 & $+0.456$\sig \ci{$+0.278$, $+0.637$} & $+0.422$\sig \ci{$+0.226$, $+0.637$} & $+0.588$\sig \ci{$+0.411$, $+0.768$} \\
 & Q4 sharpest (3.29--11.86) & 4.93 & 3.883 & 3.771 & 3.931 & 3.743 & 4.010 & 4.118 & 4.136 & $+0.365$\sig \ci{$+0.160$, $+0.553$} & $+0.205$\sig \ci{$+0.006$, $+0.426$} & $+0.393$\sig \ci{$+0.178$, $+0.607$} \\
\midrule
\scand & Q1 straightest (0.01--0.07) & 0.55 & 0.782 & 0.791 & 0.814 & 0.781 & 1.077 & 1.048 & 1.045 & $+0.254$\sig \ci{$+0.182$, $+0.316$} & $+0.231$\sig \ci{$+0.166$, $+0.298$} & $+0.264$\sig \ci{$+0.205$, $+0.322$} \\
 & Q2 (0.07--0.18) & 0.75 & 1.010 & 0.943 & 0.917 & 0.957 & 1.179 & 1.185 & 1.172 & $+0.229$\sig \ci{$+0.168$, $+0.295$} & $+0.255$\sig \ci{$+0.180$, $+0.330$} & $+0.214$\sig \ci{$+0.140$, $+0.292$} \\
 & Q3 (0.18--0.54) & 0.75 & 0.976 & 0.972 & 0.951 & 0.967 & 1.109 & 1.124 & 1.128 & $+0.156$\sig \ci{$+0.086$, $+0.223$} & $+0.177$\sig \ci{$+0.107$, $+0.252$} & $+0.161$\sig \ci{$+0.085$, $+0.237$} \\
 & Q4 sharpest (0.54--5.11) & 1.29 & 1.381 & 1.335 & 1.304 & 1.309 & 1.552 & 1.562 & 1.548 & $+0.212$\sig \ci{$+0.122$, $+0.295$} & $+0.243$\sig \ci{$+0.148$, $+0.327$} & $+0.239$\sig \ci{$+0.143$, $+0.324$} \\
