# Supplementary material for: Fewer Steps, Better Plans: Sampling Variance in Flow-Matching Navigation World Models
Source: arXiv:2611.36153 source file (2026-11-26)
Supplement: Supplementary file 26 [file supp_t2_seed1_ci_body.tex]

\multicolumn{4}{@{}l}{\emph{(a) Granularity at a fixed step count, training seed 1}} \\
\M{1}@50 $-$ {\mono}@50 & $-0.001$ [$-0.028$, $+0.028$] & $-0.065$\sig [$-0.133$, $-0.000$] & $-0.023$ [$-0.052$, $+0.003$] \\
\M{1}@5 $-$ {\mono}@5 & $-0.018$ [$-0.042$, $+0.008$] & $-0.038$ [$-0.101$, $+0.023$] & $-0.033$\sig [$-0.059$, $-0.007$] \\
\M{1}@3 $-$ {\mono}@3 & $-0.019$ [$-0.042$, $+0.008$] & $+0.002$ [$-0.069$, $+0.074$] & $-0.075$\sig [$-0.104$, $-0.048$] \\
\M{1}@2 $-$ {\mono}@2 & $+0.008$ [$-0.022$, $+0.037$] & $-0.042$ [$-0.128$, $+0.047$] & $-0.091$\sig [$-0.126$, $-0.058$] \\
\M{1}@3 (2 draws) $-$ {\mono}@3 (2 draws) & $-0.015$ [$-0.039$, $+0.009$] & $-0.017$ [$-0.085$, $+0.053$] & $-0.060$\sig [$-0.090$, $-0.032$] \\
\midrule
\multicolumn{4}{@{}l}{\emph{(b) Granularity at a fixed step count, training seed 0 (primary runs; as in \cref{tab:s-pooled})}} \\
\M{1}@50 $-$ {\mono}@50 & $+0.005$ [$-0.021$, $+0.032$] & $-0.002$ [$-0.064$, $+0.053$] & $-0.012$ [$-0.036$, $+0.013$] \\
\M{1}@5 $-$ {\mono}@5 & $-0.029$\sig [$-0.054$, $-0.004$] & $-0.008$ [$-0.065$, $+0.052$] & $-0.021$ [$-0.044$, $+0.003$] \\
\M{1}@3 $-$ {\mono}@3 & $-0.024$ [$-0.049$, $+0.001$] & $+0.053$ [$-0.009$, $+0.113$] & $-0.060$\sig [$-0.090$, $-0.033$] \\
\M{1}@2 $-$ {\mono}@2 & $-0.015$ [$-0.044$, $+0.016$] & $+0.102$\sig [$+0.032$, $+0.175$] & $-0.098$\sig [$-0.128$, $-0.069$] \\
\midrule
\multicolumn{4}{@{}l}{\emph{(c) Step reduction, training seed 1}} \\
\M{1}@5 $-$ \M{1}@50 & $-0.087$\sig [$-0.116$, $-0.061$] & $-0.100$\sig [$-0.149$, $-0.053$] & $-0.001$ [$-0.024$, $+0.019$] \\
\M{1}@3 $-$ \M{1}@50 & $-0.132$\sig [$-0.168$, $-0.099$] & $-0.090$\sig [$-0.150$, $-0.030$] & $-0.022$ [$-0.050$, $+0.003$] \\
\M{1}@2 $-$ \M{1}@50 & $-0.115$\sig [$-0.154$, $-0.081$] & $-0.099$\sig [$-0.179$, $-0.020$] & $-0.030$\sig [$-0.057$, $-0.002$] \\
{\mono}@5 $-$ {\mono}@50 & $-0.069$\sig [$-0.095$, $-0.046$] & $-0.128$\sig [$-0.175$, $-0.075$] & $+0.009$ [$-0.014$, $+0.032$] \\
{\mono}@3 $-$ {\mono}@50 & $-0.114$\sig [$-0.145$, $-0.084$] & $-0.157$\sig [$-0.217$, $-0.098$] & $+0.029$\sig [$+0.003$, $+0.057$] \\
{\mono}@2 $-$ {\mono}@50 & $-0.123$\sig [$-0.163$, $-0.088$] & $-0.122$\sig [$-0.197$, $-0.051$] & $+0.038$\sig [$+0.007$, $+0.071$] \\
{\mono}@3 (2 draws) $-$ {\mono}@50 & $-0.122$\sig [$-0.152$, $-0.093$] & $-0.232$\sig [$-0.295$, $-0.169$] & $+0.023$ [$-0.003$, $+0.050$] \\
\M{1}@5 $-$ {\mono}@50 & $-0.087$\sig [$-0.116$, $-0.058$] & $-0.165$\sig [$-0.227$, $-0.100$] & $-0.025$ [$-0.055$, $+0.005$] \\
\M{1}@2 $-$ {\mono}@50 & $-0.115$\sig [$-0.153$, $-0.083$] & $-0.164$\sig [$-0.261$, $-0.069$] & $-0.054$\sig [$-0.085$, $-0.022$] \\
\M{1}@3 (2 draws) $-$ {\mono}@50 & $-0.138$\sig [$-0.171$, $-0.105$] & $-0.249$\sig [$-0.322$, $-0.174$] & $-0.037$\sig [$-0.066$, $-0.008$] \\
\M{1}@3 (2 draws) $-$ \M{1}@3 & $-0.005$ [$-0.020$, $+0.010$] & $-0.094$\sig [$-0.135$, $-0.050$] & $+0.009$ [$-0.009$, $+0.029$] \\
{\mono}@3 (2 draws) $-$ {\mono}@3 & $-0.008$ [$-0.023$, $+0.008$] & $-0.075$\sig [$-0.112$, $-0.039$] & $-0.006$ [$-0.022$, $+0.011$] \\
\midrule
\multicolumn{4}{@{}l}{\emph{(d) Training seed 1 minus training seed 0, same model and $S$}} \\
\M{1}@50 & $+0.009$ [$-0.015$, $+0.037$] & $+0.008$ [$-0.044$, $+0.063$] & $-0.014$ [$-0.037$, $+0.010$] \\
\M{1}@5 & $+0.024$\sig [$+0.001$, $+0.049$] & $-0.005$ [$-0.066$, $+0.053$] & $+0.000$ [$-0.026$, $+0.025$] \\
\M{1}@3 & $-0.002$ [$-0.024$, $+0.024$] & $+0.039$ [$-0.024$, $+0.104$] & $-0.008$ [$-0.031$, $+0.016$] \\
\M{1}@2 & $+0.013$ [$-0.013$, $+0.041$] & $-0.066$ [$-0.136$, $+0.004$] & $-0.015$ [$-0.041$, $+0.014$] \\
\M{1}@3 (2 draws) & $-0.000$ [$-0.024$, $+0.023$] & $+0.033$ [$-0.028$, $+0.096$] & $-0.005$ [$-0.031$, $+0.024$] \\
{\mono}@50 & $+0.015$ [$-0.013$, $+0.040$] & $+0.071$\sig [$+0.015$, $+0.130$] & $-0.002$ [$-0.028$, $+0.024$] \\
{\mono}@5 & $+0.013$ [$-0.009$, $+0.033$] & $+0.024$ [$-0.029$, $+0.084$] & $+0.013$ [$-0.012$, $+0.036$] \\
{\mono}@3 & $-0.007$ [$-0.031$, $+0.017$] & $+0.090$\sig [$+0.023$, $+0.152$] & $+0.006$ [$-0.020$, $+0.033$] \\
{\mono}@2 & $-0.010$ [$-0.038$, $+0.019$] & $+0.078$\sig [$+0.004$, $+0.149$] & $-0.021$ [$-0.050$, $+0.009$] \\
\midrule
\multicolumn{4}{@{}l}{\emph{(e) Difference of contrasts between training seeds (seed 1 minus seed 0)}} \\
(\M{1}@2 $-$ {\mono}@50) & $-0.002$ [$-0.037$, $+0.035$] & $-0.137$\sig [$-0.235$, $-0.048$] & $-0.012$ [$-0.049$, $+0.027$] \\
(\M{1}@5 $-$ {\mono}@50) & $+0.009$ [$-0.025$, $+0.043$] & $-0.076$ [$-0.157$, $+0.002$] & $+0.003$ [$-0.034$, $+0.038$] \\
(\M{1}@5 $-$ \M{1}@50) & $+0.015$ [$-0.017$, $+0.047$] & $-0.013$ [$-0.078$, $+0.047$] & $+0.014$ [$-0.016$, $+0.043$] \\
({\mono}@5 $-$ {\mono}@50) & $-0.002$ [$-0.033$, $+0.029$] & $-0.047$ [$-0.112$, $+0.014$] & $+0.015$ [$-0.016$, $+0.046$] \\
