# Supplementary material for: Fewer Steps, Better Plans: Sampling Variance in Flow-Matching Navigation World Models
Source: arXiv:2611.36153 source file (2026-11-26)
Supplement: Supplementary file 27 [file supp_t2_seed1_gen_body.tex]

\recon & \mono & 50 (49) & 0.3736 & 0.4523 & 0.4133 & 0.4716 & 18.86 & 18.42 & 0.3734 & 0.4518 & 0.4127 & 0.4714 & 18.62 & 18.59 \\
 & \paper \M{4} & 50 (49) & 0.3794 & 0.4569 & 0.4184 & 0.4761 & 19.09 & 19.07 & 0.3804 & 0.4574 & 0.4187 & 0.4762 & 19.53 & 19.10 \\
 & \paper \M{1} & 50 (49) & 0.3846 & 0.4602 & 0.4221 & 0.4783 & 20.29 & 20.26 & 0.3855 & 0.4620 & 0.4216 & 0.4782 & 20.94 & 20.87 \\
 & \mono & 5 (4) & 0.3694 & 0.4531 & 0.3919 & 0.4535 & 21.69 & 21.81 & 0.3678 & 0.4519 & 0.3912 & 0.4536 & 21.96 & 21.57 \\
 & \paper \M{4} & 5 (4) & 0.3753 & 0.4582 & 0.3966 & 0.4575 & 22.91 & 22.85 & 0.3759 & 0.4582 & 0.3967 & 0.4573 & 23.13 & 22.88 \\
 & \paper \M{1} & 5 (4) & 0.3819 & 0.4627 & 0.4010 & 0.4604 & 25.00 & 24.98 & 0.3825 & 0.4641 & 0.4007 & 0.4604 & 25.35 & 25.55 \\
\midrule
\sacson & \mono & 50 (49) & 0.3232 & 0.3605 & 0.3452 & 0.3775 & 16.51 & 17.82 & 0.3230 & 0.3601 & 0.3445 & 0.3775 & 16.69 & 17.47 \\
 & \paper \M{4} & 50 (49) & 0.3331 & 0.3692 & 0.3535 & 0.3853 & 17.08 & 18.69 & 0.3324 & 0.3696 & 0.3534 & 0.3853 & 17.27 & 18.75 \\
 & \paper \M{1} & 50 (49) & 0.3433 & 0.3786 & 0.3618 & 0.3916 & 19.12 & 20.96 & 0.3423 & 0.3786 & 0.3607 & 0.3910 & 18.78 & 20.63 \\
 & \mono & 5 (4) & 0.3103 & 0.3470 & 0.3258 & 0.3580 & 20.49 & 22.45 & 0.3108 & 0.3471 & 0.3257 & 0.3582 & 20.68 & 22.14 \\
 & \paper \M{4} & 5 (4) & 0.3202 & 0.3555 & 0.3348 & 0.3661 & 21.64 & 23.67 & 0.3200 & 0.3553 & 0.3347 & 0.3656 & 21.88 & 23.89 \\
 & \paper \M{1} & 5 (4) & 0.3313 & 0.3654 & 0.3438 & 0.3739 & 24.70 & 26.61 & 0.3302 & 0.3643 & 0.3430 & 0.3727 & 24.40 & 26.87 \\
\midrule
\scand & \mono & 50 (49) & 0.4053 & 0.4565 & 0.4583 & 0.5087 & 28.55 & 31.28 & 0.4080 & 0.4579 & 0.4601 & 0.5107 & 29.29 & 32.02 \\
 & \paper \M{4} & 50 (49) & 0.3991 & 0.4580 & 0.4548 & 0.5122 & 29.05 & 32.78 & 0.4010 & 0.4579 & 0.4560 & 0.5114 & 29.53 & 33.55 \\
 & \paper \M{1} & 50 (49) & 0.3991 & 0.4587 & 0.4564 & 0.5151 & 31.12 & 35.65 & 0.4014 & 0.4594 & 0.4568 & 0.5134 & 31.53 & 35.94 \\
 & \mono & 5 (4) & 0.3975 & 0.4500 & 0.4438 & 0.4959 & 33.26 & 35.46 & 0.3998 & 0.4519 & 0.4453 & 0.4977 & 34.02 & 36.66 \\
 & \paper \M{4} & 5 (4) & 0.3887 & 0.4501 & 0.4378 & 0.4974 & 34.10 & 37.32 & 0.3905 & 0.4503 & 0.4390 & 0.4972 & 34.36 & 38.07 \\
 & \paper \M{1} & 5 (4) & 0.3894 & 0.4517 & 0.4399 & 0.5010 & 36.42 & 41.35 & 0.3913 & 0.4521 & 0.4402 & 0.4997 & 36.89 & 41.83 \\
\midrule
Three-dataset mean & \mono & 50 (49) & 0.3674 & 0.4231 & 0.4056 & 0.4526 & 21.30 & 22.51 & 0.3681 & 0.4233 & 0.4058 & 0.4532 & 21.54 & 22.70 \\
 & \paper \M{4} & 50 (49) & 0.3705 & 0.4280 & 0.4089 & 0.4579 & 21.74 & 23.51 & 0.3713 & 0.4283 & 0.4094 & 0.4577 & 22.11 & 23.80 \\
 & \paper \M{1} & 50 (49) & 0.3757 & 0.4325 & 0.4134 & 0.4617 & 23.51 & 25.62 & 0.3764 & 0.4333 & 0.4131 & 0.4609 & 23.75 & 25.81 \\
 & \mono & 5 (4) & 0.3590 & 0.4167 & 0.3872 & 0.4358 & 25.15 & 26.57 & 0.3595 & 0.4170 & 0.3874 & 0.4365 & 25.56 & 26.79 \\
 & \paper \M{4} & 5 (4) & 0.3614 & 0.4213 & 0.3897 & 0.4403 & 26.22 & 27.95 & 0.3622 & 0.4213 & 0.3901 & 0.4400 & 26.46 & 28.28 \\
 & \paper \M{1} & 5 (4) & 0.3675 & 0.4266 & 0.3949 & 0.4451 & 28.71 & 30.98 & 0.3680 & 0.4268 & 0.3946 & 0.4442 & 28.88 & 31.42 \\
