# Supplementary material for: Fewer Steps, Better Plans: Sampling Variance in Flow-Matching Navigation World Models
Source: arXiv:2611.36153 source file (2026-11-26)
Supplement: Supplementary file 28 [file supp_t2_seed1_plan_body.tex]

\multicolumn{8}{@{}l}{\emph{Training seed 1}} \\
\mono & 50 (49) & $1.378\pm0.019$ & $2.909\pm0.017$ & $1.035\pm0.017$ & $0.370\pm0.004$ & $0.714\pm0.002$ & $0.288\pm0.002$ \\
 & 5 (4) & $1.308\pm0.025$ & $2.781\pm0.015$ & $1.044\pm0.021$ & $0.366\pm0.003$ & $0.700\pm0.003$ & $0.290\pm0.001$ \\
 & 3 (2) & $1.264\pm0.006$ & $2.752\pm0.023$ & $1.064\pm0.005$ & $0.363\pm0.002$ & $0.698\pm0.003$ & $0.293\pm0.001$ \\
 & 2 (1) & $1.255\pm0.005$ & $2.787\pm0.066$ & $1.073\pm0.017$ & $0.366\pm0.003$ & $0.702\pm0.010$ & $0.294\pm0.004$ \\
 & $2{\times}3$ ($2{\times}2$) & $1.255\pm0.012$ & $2.677\pm0.010$ & $1.059\pm0.003$ & -- & -- & -- \\
\paper \M{1} & 50 (49) & $1.377\pm0.035$ & $2.843\pm0.021$ & $1.012\pm0.016$ & $0.367\pm0.007$ & $0.697\pm0.006$ & $0.283\pm0.003$ \\
 & 5 (4) & $1.290\pm0.011$ & $2.743\pm0.001$ & $1.011\pm0.022$ & $0.365\pm0.001$ & $0.691\pm0.007$ & $0.283\pm0.001$ \\
 & 3 (2) & $1.245\pm0.004$ & $2.754\pm0.040$ & $0.990\pm0.038$ & $0.367\pm0.001$ & $0.692\pm0.006$ & $0.281\pm0.005$ \\
 & 2 (1) & $1.262\pm0.005$ & $2.745\pm0.017$ & $0.982\pm0.029$ & $0.375\pm0.001$ & $0.690\pm0.008$ & $0.281\pm0.002$ \\
 & $2{\times}3$ ($2{\times}2$) & $1.240\pm0.014$ & $2.660\pm0.029$ & $0.999\pm0.012$ & -- & -- & -- \\
\midrule
\multicolumn{8}{@{}l}{\emph{Training seed 0 (primary runs, for reference)}} \\
\mono & 50 (49) & $1.363\pm0.010$ & $2.838\pm0.024$ & $1.038\pm0.023$ & $0.367\pm0.001$ & $0.698\pm0.003$ & $0.288\pm0.002$ \\
 & 5 (4) & $1.295\pm0.013$ & $2.756\pm0.034$ & $1.032\pm0.023$ & $0.363\pm0.003$ & $0.690\pm0.003$ & $0.287\pm0.002$ \\
 & 3 (2) & $1.271\pm0.017$ & $2.662\pm0.059$ & $1.058\pm0.015$ & $0.366\pm0.003$ & $0.683\pm0.007$ & $0.292\pm0.002$ \\
 & 2 (1) & $1.265\pm0.003$ & $2.708\pm0.039$ & $1.094\pm0.015$ & $0.371\pm0.003$ & $0.685\pm0.001$ & $0.297\pm0.002$ \\
\paper \M{1} & 50 (49) & $1.368\pm0.024$ & $2.836\pm0.059$ & $1.026\pm0.015$ & $0.367\pm0.003$ & $0.694\pm0.010$ & $0.285\pm0.002$ \\
 & 5 (4) & $1.266\pm0.016$ & $2.749\pm0.077$ & $1.011\pm0.014$ & $0.363\pm0.001$ & $0.692\pm0.015$ & $0.283\pm0.001$ \\
 & 3 (2) & $1.247\pm0.004$ & $2.715\pm0.036$ & $0.997\pm0.022$ & $0.370\pm0.001$ & $0.688\pm0.005$ & $0.282\pm0.002$ \\
 & 2 (1) & $1.249\pm0.010$ & $2.811\pm0.027$ & $0.996\pm0.012$ & $0.376\pm0.003$ & $0.705\pm0.005$ & $0.284\pm0.002$ \\
 & $2{\times}3$ ($2{\times}2$) & $1.240\pm0.005$ & $2.627\pm0.031$ & $1.003\pm0.032$ & -- & -- & -- \\
