# Supplementary material for: Fewer Steps, Better Plans: Sampling Variance in Flow-Matching Navigation World Models
Source: arXiv:2611.36153 source file (2026-11-26)
Supplement: Supplementary file 29 [file supp_turns_body.tex]

\recon & Q1 straightest (0.07--1.14) & 0.89 & 0.81 & 1.09 & 1.08 & 1.08 & 1.08 & 1.06 & 1.05 & 1.05 & $0.00$ \ci{$-0.04$, $+0.04$} & $-0.02$ \ci{$-0.06$, $+0.03$} & $-0.03$ \ci{$-0.07$, $+0.03$} & $-0.03$ \ci{$-0.09$, $+0.03$} & $+0.01$ \ci{$-0.04$, $+0.04$} & $-0.01$ \ci{$-0.04$, $+0.03$} \\
 & Q2 (1.15--2.20) & 1.25 & 1.17 & 1.16 & 1.10 & 1.17 & 1.13 & 1.11 & 1.12 & 1.14 & $-0.03$ \ci{$-0.08$, $+0.02$} & $-0.05$\sig \ci{$-0.10$, $-0.00$} & $+0.01$ \ci{$-0.04$, $+0.05$} & $-0.03$ \ci{$-0.08$, $+0.03$} & $-0.02$ \ci{$-0.06$, $+0.01$} & $-0.06$\sig \ci{$-0.10$, $-0.01$} \\
 & Q3 (2.20--3.53) & 1.73 & 1.69 & 1.31 & 1.24 & 1.28 & 1.16 & 1.15 & 1.14 & 1.17 & $-0.12$\sig \ci{$-0.16$, $-0.07$} & $-0.13$\sig \ci{$-0.18$, $-0.08$} & $+0.02$ \ci{$-0.03$, $+0.06$} & $-0.10$\sig \ci{$-0.16$, $-0.04$} & $-0.03$ \ci{$-0.07$, $+0.01$} & $-0.08$\sig \ci{$-0.13$, $-0.03$} \\
 & Q4 sharpest (3.54--8.95) & 2.68 & 2.68 & 1.89 & 1.76 & 1.95 & 1.70 & 1.67 & 1.65 & 1.64 & $-0.25$\sig \ci{$-0.31$, $-0.19$} & $-0.28$\sig \ci{$-0.35$, $-0.21$} & $-0.06$ \ci{$-0.14$, $+0.01$} & $-0.31$\sig \ci{$-0.40$, $-0.22$} & $+0.01$ \ci{$-0.04$, $+0.07$} & $-0.13$\sig \ci{$-0.18$, $-0.07$} \\
\midrule
\sacson & Q1 straightest (0.00--0.60) & 2.67 & 1.19 & 1.75 & 1.65 & 1.72 & 1.64 & 1.54 & 1.47 & 1.69 & $-0.07$ \ci{$-0.15$, $+0.01$} & $-0.18$\sig \ci{$-0.28$, $-0.09$} & $+0.04$ \ci{$-0.08$, $+0.16$} & $-0.03$ \ci{$-0.17$, $+0.12$} & $-0.22$\sig \ci{$-0.35$, $-0.12$} & $-0.09$\sig \ci{$-0.17$, $-0.02$} \\
 & Q2 (0.61--1.49) & 3.60 & 1.65 & 2.69 & 2.66 & 2.76 & 2.69 & 2.64 & 2.54 & 2.70 & $-0.07$ \ci{$-0.16$, $+0.04$} & $-0.12$ \ci{$-0.23$, $+0.00$} & $+0.01$ \ci{$-0.12$, $+0.14$} & $-0.05$ \ci{$-0.21$, $+0.09$} & $-0.16$\sig \ci{$-0.27$, $-0.05$} & $-0.04$ \ci{$-0.12$, $+0.06$} \\
 & Q3 (1.51--3.28) & 3.92 & 2.31 & 3.03 & 2.93 & 3.00 & 2.89 & 2.88 & 2.76 & 2.92 & $-0.11$\sig \ci{$-0.21$, $-0.01$} & $-0.12$ \ci{$-0.24$, $+0.00$} & $+0.03$ \ci{$-0.11$, $+0.17$} & $-0.07$ \ci{$-0.22$, $+0.08$} & $-0.17$\sig \ci{$-0.28$, $-0.05$} & $-0.10$\sig \ci{$-0.20$, $-0.00$} \\
 & Q4 sharpest (3.29--11.86) & 4.93 & 3.82 & 3.88 & 3.79 & 3.87 & 3.77 & 3.80 & 3.74 & 3.93 & $-0.10$ \ci{$-0.19$, $+0.00$} & $-0.07$ \ci{$-0.21$, $+0.06$} & $+0.16$\sig \ci{$+0.01$, $+0.32$} & $+0.06$ \ci{$-0.11$, $+0.24$} & $-0.19$\sig \ci{$-0.32$, $-0.06$} & $-0.09$ \ci{$-0.19$, $+0.01$} \\
\midrule
\scand & Q1 straightest (0.01--0.07) & 0.55 & 0.55 & 0.78 & 0.79 & 0.78 & 0.79 & 0.80 & 0.78 & 0.81 & $+0.01$ \ci{$-0.03$, $+0.05$} & $+0.01$ \ci{$-0.04$, $+0.06$} & $+0.02$ \ci{$-0.03$, $+0.07$} & $+0.03$ \ci{$-0.02$, $+0.08$} & $-0.03$ \ci{$-0.07$, $+0.01$} & $0.00$ \ci{$-0.04$, $+0.04$} \\
 & Q2 (0.07--0.18) & 0.75 & 0.75 & 1.01 & 1.00 & 0.97 & 0.94 & 0.93 & 0.96 & 0.92 & $-0.03$ \ci{$-0.08$, $+0.01$} & $-0.04$ \ci{$-0.09$, $+0.01$} & $-0.03$ \ci{$-0.08$, $+0.02$} & $-0.06$ \ci{$-0.12$, $+0.00$} & $+0.04$ \ci{$-0.01$, $+0.09$} & $-0.01$ \ci{$-0.05$, $+0.03$} \\
 & Q3 (0.18--0.54) & 0.75 & 0.75 & 0.98 & 0.97 & 1.01 & 0.97 & 0.95 & 0.97 & 0.95 & $-0.04$ \ci{$-0.08$, $+0.01$} & $-0.06$\sig \ci{$-0.11$, $-0.01$} & $-0.02$ \ci{$-0.08$, $+0.03$} & $-0.06$\sig \ci{$-0.12$, $-0.00$} & $+0.02$ \ci{$-0.03$, $+0.06$} & $-0.01$ \ci{$-0.05$, $+0.04$} \\
 & Q4 sharpest (0.54--5.11) & 1.29 & 1.29 & 1.38 & 1.37 & 1.33 & 1.34 & 1.31 & 1.31 & 1.30 & $0.00$ \ci{$-0.05$, $+0.05$} & $-0.02$ \ci{$-0.07$, $+0.03$} & $-0.03$ \ci{$-0.08$, $+0.02$} & $-0.03$ \ci{$-0.09$, $+0.03$} & $0.00$ \ci{$-0.04$, $+0.05$} & $-0.02$ \ci{$-0.06$, $+0.03$} \\
